# Supplementary material for: Adaptive Multipath-Based SLAM for Distributed MIMO Systems
Source: arXiv:2506.21798 source file (2026-03-27)
Supplement: Supplementary file 1 [file supplementary.pdf]

# Adaptive Multipath-Based SLAM for Distributed MIMO Systems: Supporting Document

Xuhong Li, Benjamin Deutschmann, Erik Leitinger, and Florian Meyer

This manuscript provides derivations of the statistical models and the sum-product algorithm (SPA) for the publication, “Adaptive Multipath-Based SLAM for Distributed MIMO Systems” by the same authors [1].

## I. STATISTICAL MODEL

In this section, we derive the joint posterior probability density function (PDF)  $f(\mathbf{x}_{0:n}, \mathbf{y}_{0:n}, \boldsymbol{\beta}_{0:n}, \underline{\mathbf{a}}_{1:n}, \bar{\mathbf{a}}_{1:n}, \mathbf{m}_{1:n} | \mathbf{z}_{1:n})$ . At first, a few sets are defined as follows:  $\mathcal{M}_n^{(j)} \triangleq \{1, \dots, M_n^{(j)}\}$  denotes the sets of measurement indexes,  $\mathcal{N}_n^{(j)} \triangleq \{m \in \mathcal{M}_n^{(j)} : \bar{r}_{m,n}^{(j)} = 1, \bar{r}_{mm,n}^{(j)} = 1, \bar{a}_{m,n}^{(j)} = 0\}$  denotes the set of existing new potential surface feature vectors (SFVs) and corresponding potential rays (PRs),  $\mathcal{Q}_n^{(j)} \triangleq \{(s, s') \in \tilde{\mathcal{D}}_n^{(j)} : \underline{r}_{s,n}^{(j)} = 1, \underline{r}_{s',n}^{(j)} = 1, \underline{r}_{ss',n}^{(j)} = 1, \underline{a}_{ss',n}^{(j)} \in \mathcal{M}_n^{(j)}\}$  denotes the sets of existing legacy potential SFVs (PSFVs) and corresponding PRs. We further define  $\mathcal{M}_{0,n}^{(j)} \triangleq \{0, \mathcal{M}_n^{(j)}\}$ .

### A. Joint Prior PDF

The joint prior PDF of  $\mathbf{x}_{0:n}, \mathbf{y}_{0:n}, \boldsymbol{\beta}_{0:n}, \underline{\mathbf{a}}_{1:n}, \bar{\mathbf{a}}_{1:n}$  and the number of measurements  $\mathbf{m}_{1:n}$  factorizes as

$$\begin{aligned}
 & f(\mathbf{x}_{0:n}, \mathbf{y}_{0:n}, \boldsymbol{\beta}_{0:n}, \underline{\mathbf{a}}_{1:n}, \bar{\mathbf{a}}_{1:n}, \mathbf{m}_{1:n}) \\
 &= f(\mathbf{x}_{0:n}, \underline{\mathbf{y}}_{0:n}, \underline{\boldsymbol{\beta}}_{0:n}, \bar{\boldsymbol{\beta}}_{1:n}, \underline{\mathbf{a}}_{1:n}, \bar{\mathbf{a}}_{1:n}, \mathbf{m}_{1:n}) \\
 &= \underbrace{\left( f(\mathbf{x}_0) \prod_{s=1}^{S_0} f(\mathbf{y}_{s,0}) \prod_{j'=1}^J \prod_{(s,s') \in \tilde{\mathcal{D}}_0^{(j')}} f(\boldsymbol{\beta}_{ss',0}^{(j')}) \right)}_{\text{initial prior PDFs}} \underbrace{\prod_{n'=1}^n f(\mathbf{x}_{n'} | \mathbf{x}_{n'-1})}_{\text{agent state transition}} \\
 &\quad \times \underbrace{\left( \prod_{s'=1}^{S_{n'-1}} f(\underline{\mathbf{y}}_{s',n'} | \mathbf{y}_{s',n'-1}) \right) \left( \prod_{j'=2}^J \prod_{s'=1}^{S_{n'}^{(j')}} f^{(j)}(\underline{\mathbf{y}}_{s',n'}^{(j')} | \mathbf{y}_{s',n'}^{(j'-1)}) \right)}_{\text{legacy PSFVs state transition}} \underbrace{\left( \prod_{j''=1}^J \prod_{(s,s') \in \tilde{\mathcal{D}}_{n'}^{(j'')}} f(\underline{\boldsymbol{\beta}}_{ss',n'}^{(j'')} | \boldsymbol{\beta}_{ss',n'-1}^{(j'')}) \right)}_{\text{legacy PRs state transition}} \\
 &\quad \times \prod_{j=1}^J f(\bar{\mathbf{p}}_{\text{sfv}}^{(j)}, \bar{\mathbf{u}}_{n'}^{(j)} | \bar{\mathbf{r}}_{n'}^{(j)}, \bar{\mathbf{r}}_{n'}^{(j)}, M_{n'}^{(j)}, \mathbf{x}_{n'}) p(\bar{\mathbf{r}}_{n'}^{(j)}, \bar{\mathbf{r}}_{n'}^{(j)}, \underline{\mathbf{a}}_{n'}^{(j)}, \bar{\mathbf{a}}_{n'}^{(j)}, M_{n'}^{(j)} | \mathbf{y}_{n'}^{(j)}, \boldsymbol{\beta}_{n'}^{(j)}, \mathbf{x}_{n'}). \tag{1}
 \end{aligned}$$

The joint prior PDF of new PSFVs and new PRs  $f(\bar{\mathbf{p}}_{\text{sfv}}^{(j)}, \bar{\mathbf{u}}_{n'}^{(j)} | \bar{\mathbf{r}}_{n'}^{(j)}, \bar{\mathbf{r}}_{n'}^{(j)}, M_{n'}^{(j)}, \mathbf{x}_{n'})$  and the joint conditional prior probability mass function (PMF)  $p(\bar{\mathbf{r}}_{n'}^{(j)}, \bar{\mathbf{r}}_{n'}^{(j)}, \underline{\mathbf{a}}_{n'}^{(j)}, \bar{\mathbf{a}}_{n'}^{(j)}, M_{n'}^{(j)} | \mathbf{y}_{n'}^{(j)}, \boldsymbol{\beta}_{n'}^{(j)}, \mathbf{x}_{n'})$  are further defined as follows.

The joint prior PDF of new PSFVs and new PRs  $f(\bar{\mathbf{p}}_{\text{sfv}}^{(j)}, \bar{\mathbf{u}}_{n'}^{(j)} | \bar{\mathbf{r}}_{n'}^{(j)}, \bar{\mathbf{r}}_{n'}^{(j)}, M_{n'}^{(j)}, \mathbf{x}_{n'})$  is given as

$$f(\bar{\mathbf{p}}_{\text{sfv}}^{(j)}, \bar{\mathbf{u}}_{n'}^{(j)} | \bar{\mathbf{r}}_{n'}^{(j)}, \bar{\mathbf{r}}_{n'}^{(j)}, M_{n'}^{(j)}, \mathbf{x}_{n'}) = \prod_{m \in \mathcal{N}_n^{(j)}} f_{\text{n}}(\bar{\mathbf{p}}_{m,\text{sfv}}^{(j)}, \bar{\mathbf{u}}_{mm,n}^{(j)} | \mathbf{x}_n) \prod_{m' \in \mathcal{M}_n^{(j)} \setminus \mathcal{N}_n^{(j)}} f_{\text{D}}(\bar{\mathbf{p}}_{m',\text{sfv}}^{(j)}) f_{\text{D}}(\bar{\mathbf{u}}_{m'm',n}^{(j)}). \tag{2}$$

The joint conditional prior PMF  $p(\bar{\mathbf{r}}_n^{(j)}, \bar{\mathbf{r}}_n^{(j)}, \underline{\mathbf{a}}_n^{(j)}, \bar{\mathbf{a}}_n^{(j)}, M_n^{(j)} | \underline{\mathbf{y}}_n^{(j)}, \underline{\boldsymbol{\beta}}_n^{(j)}, \mathbf{x}_n)$  is given as

$$\begin{aligned}
& p(\bar{\mathbf{r}}_n^{(j)}, \bar{\mathbf{r}}_n^{(j)}, \underline{\mathbf{a}}_n^{(j)}, \bar{\mathbf{a}}_n^{(j)}, M_n^{(j)} | \underline{\mathbf{y}}_n^{(j)}, \underline{\boldsymbol{\beta}}_n^{(j)}, \mathbf{x}_n) \\
&= \chi_{\bar{\mathbf{r}}_n^{(j)}, \underline{\mathbf{a}}_n^{(j)}, M_n^{(j)}} \underbrace{\left( \prod_{m \in \mathcal{N}_n^{(j)}} \Gamma_{\underline{\mathbf{a}}_n^{(j)}}(\bar{\mathbf{r}}_{m,n}^{(j)}, \bar{\mathbf{r}}_{mm,n}^{(j)}) \right)}_{\text{exclusion functions}} \left( \prod_{(s,s') \in \tilde{\mathcal{D}}_n^{(j)}} \Gamma_{\underline{\mathbf{a}}_n^{(j)}}(\underline{r}_{s,n}^{(j)}, \underline{r}_{s',n}^{(j)}, \underline{r}_{ss',n}^{(j)}) \right) \\
&\times \underbrace{\prod_{(s,s') \in \tilde{\mathcal{D}}_n^{(j)}} \prod_{m=1}^{M_n^{(j)}} \psi(\underline{a}_{ss',n}^{(j)}, \bar{a}_{m,n}^{(j)})}_{\text{binary check functions}} \left( \prod_{(s,s') \in \mathcal{Q}_n^{(j)}} p_d(\underline{u}_{ss',n}^{(j)}) \right) \left( \prod_{(s,s') \in \tilde{\mathcal{D}}_n^{(j)} \setminus \mathcal{Q}_n^{(j)}} 1(\underline{a}_{ss',n}^{(j)} - p_{d,ss'}(\underline{u}_{ss',n}^{(j)}) \right). \quad (3)
\end{aligned}$$

where the normalization constant  $\chi_{\bar{\mathbf{r}}_n^{(j)}, \underline{\mathbf{a}}_n^{(j)}, M_n^{(j)}}$  is defined inline with [2], the binary check function  $\psi(\underline{a}_{ss',n}^{(j)}, \bar{a}_{m,n}^{(j)})$  checks if the PSFV-oriented association variable  $\underline{a}_{ss',n}^{(j)}$  and the measurement-oriented association variable  $\bar{a}_{m,n}^{(j)}$  describe the same association event.

Based on the existence/non-existence relations between PSFVs and corresponding PRs, several invalid cases are defined. The joint prior PDF is enforce to be zero for these cases using the exclusion functions  $\Gamma_{\underline{\mathbf{a}}_n^{(j)}}(\underline{r}_{s,n}^{(j)}, \underline{r}_{s',n}^{(j)}, \underline{r}_{ss',n}^{(j)})$  and  $\Gamma_{\bar{\mathbf{a}}_n^{(j)}}(\bar{\mathbf{r}}_{m,n}^{(j)}, \bar{\mathbf{r}}_{mm,n}^{(j)})$ . Fundamentally, a PSFV models a potentially existing environmental object and PRs model signal interacting processes on this object, thus their existence/non-existence status are related as follows: (i) a nonexistent reflective surface cannot generate any propagation paths, i.e., from  $r_{s,n} = 0$  follows  $r_{ss',n}^{(j)} = 0 \forall (s, s')$ ; (ii) an existing surface does not necessarily interact with any radio frequency (RF) signals and therefore generate propagation paths, i.e., if  $r_{s,n} = 1$ , then  $r_{ss',n}^{(j)} \in \{1, 0\}$ ; (iii) a path exists if and only if the interacting surfaces all exist, i.e., from  $r_{ss',n}^{(j)} = 1$  follows  $r_{s,n} = 1$  and  $r_{s',n} = 1$ . Accordingly, the invalid cases and exclusion functions are defined in what follows.

For physical anchors (PAs) and corresponding line-of-sight (LoS) PR:  $(s, s') = (0, 0)$ , the exclusion function  $\Gamma_{\underline{\mathbf{a}}_n^{(j)}}(\underline{r}_{s,n}^{(j)}, \underline{r}_{s',n}^{(j)}, \underline{r}_{ss',n}^{(j)}) = \Gamma_{\underline{\mathbf{a}}_n^{(j)}}(\underline{r}_{00,n}^{(j)})$  is given as

$$\Gamma_{\underline{\mathbf{a}}_n^{(j)}}(\underline{r}_{00,n}^{(j)}) = \begin{cases} 1, & \underline{r}_{00,n}^{(j)} = 1, \underline{a}_{00,n}^{(j)} \in \mathcal{M}_n^{(j)} & \Rightarrow \text{Eq. (19) in [1]} \\ 1, & \underline{r}_{00,n}^{(j)} = 1, \underline{a}_{00,n}^{(j)} = 0 \\ 1, & \underline{r}_{00,n}^{(j)} = 0, \underline{a}_{00,n}^{(j)} = 0 \\ 0, & \underline{r}_{00,n}^{(j)} = 0, \underline{a}_{00,n}^{(j)} \in \mathcal{M}_n^{(j)} & \Rightarrow \text{invalid case ①} \end{cases} \quad (4)$$

where the *invalid case for LoS PR* indicates a nonexistent LoS path is associated to a measurement.

For legacy PSFVs and corresponding single-bounce PRs:  $s = s' \wedge (s, s') \neq (0, 0)$ , the exclusion function  $\Gamma_{\underline{\mathbf{a}}_n^{(j)}}(\underline{r}_{s,n}^{(j)}, \underline{r}_{s',n}^{(j)}, \underline{r}_{ss',n}^{(j)}) = \Gamma_{\underline{\mathbf{a}}_n^{(j)}}(\underline{r}_{s,n}^{(j)}, \underline{r}_{ss,n}^{(j)})$  is given as

$$\Gamma_{\underline{\mathbf{a}}_n^{(j)}}(\underline{r}_{s,n}^{(j)}, \underline{r}_{ss,n}^{(j)}) = \begin{cases} 1, & \underline{r}_{s,n}^{(j)} = 1, \underline{r}_{ss,n}^{(j)} = 1, \underline{a}_{ss,n}^{(j)} \in \mathcal{M}_{0,n}^{(j)} & \Rightarrow \text{Eq. (20) in [1]} \\ 1, & \forall \underline{r}_{s,n}^{(j)}, \underline{r}_{ss,n}^{(j)} = 0, \underline{a}_{ss,n}^{(j)} = 0 \\ 0, & \forall \underline{r}_{s,n}^{(j)}, \underline{r}_{ss,n}^{(j)} = 0, \underline{a}_{ss,n}^{(j)} \in \mathcal{M}_n^{(j)} \\ 0, & \underline{r}_{s,n}^{(j)} = 0, \underline{r}_{ss,n}^{(j)} = 1, \underline{a}_{ss,n}^{(j)} \in \mathcal{M}_{0,n}^{(j)} & \Rightarrow \text{invalid cases ②} \end{cases} \quad (5)$$

where the *invalid cases for single-bounce PRs* indicate: (i) a nonexistent single-bounce path is associated to a measurement; (ii) surface is nonexistent but the associated single-bounce path exists.

For legacy PSFVs and corresponding double-bounce PRs:  $s \neq s' \wedge (s, s') \neq (0, 0)$ , the exclusion function  $\Gamma_{\underline{\mathbf{a}}_n^{(j)}}(\underline{r}_{s,n}^{(j)}, \underline{r}_{s',n}^{(j)}, \underline{r}_{ss',n}^{(j)})$  is given as

$$\Gamma_{\underline{\mathbf{a}}_n^{(j)}}(\underline{r}_{s,n}^{(j)}, \underline{r}_{s',n}^{(j)}, \underline{r}_{ss',n}^{(j)}) = \begin{cases} 1, & \underline{r}_{s,n}^{(j)} = 1, \underline{r}_{s',n}^{(j)} = 1, \underline{r}_{ss',n}^{(j)} = 1, \underline{a}_{ss',n}^{(j)} \in \mathcal{M}_{0,n}^{(j)} & \Rightarrow \text{Eq. (21) in [1]} \\ 1, & \forall (\underline{r}_{s,n}^{(j)}, \underline{r}_{ss',n}^{(j)}), \underline{r}_{ss',n}^{(j)} = 0, \underline{a}_{ss',n}^{(j)} = 0 \\ 0, & \forall (\underline{r}_{s,n}^{(j)}, \underline{r}_{ss',n}^{(j)}), \underline{r}_{ss',n}^{(j)} = 0, \underline{a}_{ss',n}^{(j)} \in \mathcal{M}_n^{(j)} \\ 0, & (\underline{r}_{s,n}^{(j)} = 0) \vee (\underline{r}_{s',n}^{(j)} = 0), \underline{r}_{ss',n}^{(j)} = 1, \underline{a}_{ss',n}^{(j)} \in \mathcal{M}_{0,n}^{(j)} & \Rightarrow \text{invalid cases ③} \end{cases} \quad (6)$$

where the *invalid cases for double-bounce PRs* indicate: (i) a nonexistent double-bounce path is associated to a measurement; (ii) one or both surfaces are nonexistent but the associated double-bounce path exists.

For new PSFVs and corresponding PRs: the exclusion function  $\Gamma_{\underline{a}_n^{(j)}}(\bar{r}_{m,n}^{(j)}, \bar{r}_{mm,n}^{(j)})$  is defined as

$$\Gamma_{\underline{a}_n^{(j)}}(\bar{r}_{m,n}^{(j)}, \bar{r}_{mm,n}^{(j)}) = \begin{cases} 1, & \bar{r}_{m,n}^{(j)} = 1, \bar{r}_{mm,n}^{(j)} = 1, \underline{a}_{ss',n}^{(j)} = 0 \Rightarrow \text{Eq. (22) in [1]} \\ 1, & \bar{r}_{m,n}^{(j)} = 0, \bar{r}_{mm,n}^{(j)} = 0, \underline{a}_{ss',n}^{(j)} \in \mathcal{M}_{0,n}^{(j)} \\ 0, & \text{otherwise} \Rightarrow \text{invalid cases (4)} \end{cases} \quad (7)$$

where the **invalid cases for new PRs** indicate: the exclusive presence of a new PSFV and its corresponding new PR, meaning one exists while the other does not.

We further define the function  $p_{d,ss'}(\underline{u}_{ss',n}^{(j)})$  providing the detection probabilities constrained by the corresponding PSFV and PR existence probabilities, given as

$$p_{d,ss'}(\underline{u}_{ss',n}^{(j)}) \triangleq \begin{cases} \underline{r}_{00,n}^{(j)} p_d(\underline{u}_{00,n}^{(j)}), & (s, s') = (0, 0) \\ \underline{r}_{s,n}^{(j)} \underline{r}_{ss,n}^{(j)} p_d(\underline{u}_{ss,n}^{(j)}), & s = s' \wedge (s, s') \neq (0, 0) \\ \underline{r}_{s,n}^{(j)} \underline{r}_{s',n}^{(j)} \underline{r}_{ss',n}^{(j)} p_d(\underline{u}_{ss',n}^{(j)}), & s \neq s' \wedge (s, s') \neq (0, 0). \end{cases} \quad (8)$$

The product of the joint prior PDF (2) and the joint conditional prior PMF (3) can be written up to the normalization constant as

$$\begin{aligned} & f(\bar{\mathbf{p}}_{\text{sfv}}^{(j)}, \bar{\mathbf{u}}_n^{(j)} | \bar{\mathbf{r}}_n^{(j)}, \bar{\mathbf{r}}_n^{(j)}, M_n^{(j)}, \mathbf{x}_n) p(\bar{\mathbf{r}}_n^{(j)}, \bar{\mathbf{r}}_n^{(j)}, \underline{\mathbf{a}}_n^{(j)}, \bar{\mathbf{a}}_n^{(j)}, M_n^{(j)} | \underline{\mathbf{y}}_n^{(j)}, \underline{\beta}_n^{(j)}, \mathbf{x}_n) \\ & \propto \prod_{(s,s') \in \tilde{\mathcal{D}}_n^{(j)}} \prod_{m=1}^{M_n^{(j)}} \psi(\underline{a}_{ss',n}^{(j)}, \bar{a}_{m,n}^{(j)}) \\ & \times \underbrace{\left( \prod_{(s,s') \in \tilde{\mathcal{D}}_n^{(j)}} \Gamma_{\underline{a}_n^{(j)}}(\underline{r}_{s,n}^{(j)}, \underline{r}_{s',n}^{(j)}, \underline{r}_{ss',n}^{(j)}) \prod_{(s,s') \in \mathcal{Q}_n^{(j)}} \frac{p_d(\underline{u}_{ss',n}^{(j)})}{\mu_{\text{fa}}} \prod_{(s,s') \in \tilde{\mathcal{D}}_n^{(j)} \setminus \mathcal{Q}_n^{(j)}} (1(\underline{a}_{ss',n}^{(j)}) - p_{d,ss'}(\underline{u}_{ss',n}^{(j)})) \right)}_{\text{factors related to PAs, legacy PSFVs and their corresponding PRs}} \\ & \times \underbrace{\left( \prod_{m \in \mathcal{N}_n^{(j)}} \frac{\mu_n f_n(\bar{\mathbf{p}}_{m,\text{sfv}}^{(j)}, \bar{\mathbf{u}}_{mm,n}^{(j)} | \mathbf{x}_n)}{\mu_{\text{fa}}} \Gamma_{\underline{a}_n^{(j)}}(\bar{r}_{m,n}^{(j)}, \bar{r}_{mm,n}^{(j)}) \prod_{m' \in \mathcal{M}_n^{(j)} \setminus \mathcal{N}_n^{(j)}} f_D(\bar{\mathbf{p}}_{m',\text{sfv}}^{(j)}) f_D(\bar{\mathbf{u}}_{m'm',n}^{(j)}) \right)}_{\text{factors related to the new PSFVs and corresponding PRs}}. \end{aligned} \quad (9)$$

After integrating the definitions of the binary check function  $\psi(\underline{a}_{ss',n}^{(j)}, \bar{a}_{m,n}^{(j)})$ , the exclusion functions  $\Gamma_{\underline{a}_n^{(j)}}(\underline{r}_{s,n}^{(j)}, \underline{r}_{s',n}^{(j)}, \underline{r}_{ss',n}^{(j)})$  and  $\Gamma_{\underline{a}_n^{(j)}}(\bar{r}_{m,n}^{(j)}, \bar{r}_{mm,n}^{(j)})$ , and with some simple manipulations, Eq. (9) can be further written as

$$\begin{aligned} & f(\bar{\mathbf{p}}_{\text{sfv}}^{(j)}, \bar{\mathbf{u}}_n^{(j)} | \bar{\mathbf{r}}_n^{(j)}, \bar{\mathbf{r}}_n^{(j)}, M_n^{(j)}, \mathbf{x}_n) p(\bar{\mathbf{r}}_n^{(j)}, \bar{\mathbf{r}}_n^{(j)}, \underline{\mathbf{a}}_n^{(j)}, \bar{\mathbf{a}}_n^{(j)}, M_n^{(j)} | \underline{\mathbf{y}}_n^{(j)}, \underline{\beta}_n^{(j)}, \mathbf{x}_n) \\ & \propto \left( \prod_{m'=1}^{M_n^{(j)}} \psi(\underline{a}_{00,n}^{(j)}, \bar{a}_{m',n}^{(j)}) \prod_{j=1}^J q_{\text{P1}}(\underline{\beta}_{00,n}^{(j)}, \underline{a}_{00,n}^{(j)}) \right) \\ & \times \left( \prod_{m'=1}^{M_n^{(j)}} \psi(\underline{a}_{ss,n}^{(j)}, \bar{a}_{m',n}^{(j)}) \prod_{s=1}^{S_n^{(j)}} q_{\text{S1}}(\underline{\mathbf{y}}_{s,n}^{(j)}, \underline{\beta}_{ss,n}^{(j)}, \underline{a}_{ss,n}^{(j)}) \right) \\ & \times \left( \prod_{m'=1}^{M_n^{(j)}} \psi(\underline{a}_{ss',n}^{(j)}, \bar{a}_{m',n}^{(j)}) \prod_{s'=1, s' \neq s}^{S_n^{(j)}} q_{\text{D1}}(\underline{\mathbf{y}}_{s,n}^{(j)}, \underline{\mathbf{y}}_{s',n}^{(j)}, \underline{\beta}_{ss',n}^{(j)}, \underline{a}_{ss',n}^{(j)}) \right) \\ & \times \left( \prod_{m=1}^{M_n^{(j)}} \bar{q}_{\text{N1}}(\bar{\mathbf{y}}_{m,n}^{(j)}, \bar{\beta}_{m,n}^{(j)}, \bar{a}_{m,n}^{(j)}) \right). \end{aligned} \quad (10)$$

The function  $q_{\text{P1}}(\underline{\beta}_{00,n}^{(j)}, \underline{a}_{00,n}^{(j)}) = q_{\text{P1}}(\underline{u}_{00,n}^{(j)}, \underline{r}_{00,n}^{(j)}, \underline{a}_{00,n}^{(j)})$  for PAs integrating the definition of the exclusion function

$\Gamma_{\underline{a}_n^{(j)}}(r_{00,n}^{(j)})$  is given by

$$q_{P1}(\underline{u}_{00,n}^{(j)}, r_{00,n}^{(j)} = 1, \underline{a}_{00,n}^{(j)}) \triangleq \begin{cases} \frac{p_d(\underline{u}_{00,n}^{(j)})}{\mu_{fa}}, & \underline{a}_{00,n}^{(j)} \in \mathcal{M}_n^{(j)} \\ 1 - p_d(\underline{u}_{00,n}^{(j)}), & \underline{a}_{00,n}^{(j)} = 0, \end{cases} \quad (11)$$

$q_{P1}(\underline{u}_{00,n}^{(j)}, r_{00,n}^{(j)} = 0, \underline{a}_{00,n}^{(j)} = 0) = 1$ , and  $q_{P1}(\underline{u}_{00,n}^{(j)}, r_{00,n}^{(j)} = 0, \underline{a}_{00,n}^{(j)} = m) = 0$  for the *invalid case* ①.

The function  $q_{S1}(\underline{y}_{s,n}^{(j)}, \underline{\beta}_{ss,n}^{(j)}, \underline{a}_{ss,n}^{(j)}) = q_{S1}(\underline{r}_{s,n}^{(j)}, \underline{u}_{ss,n}^{(j)}, \underline{r}_{ss,n}^{(j)}, \underline{a}_{ss,n}^{(j)})$  integrating the definition of the exclusion function  $\Gamma_{\underline{a}_n^{(j)}}(\underline{r}_{s,n}^{(j)}, \underline{r}_{ss,n}^{(j)})$  is given by

$$q_{S1}(\underline{r}_{s,n}^{(j)} = 1, \underline{u}_{ss,n}^{(j)}, \underline{r}_{ss,n}^{(j)} = 1, \underline{a}_{ss,n}^{(j)}) \triangleq \begin{cases} \frac{p_d(\underline{u}_{ss,n}^{(j)})}{\mu_{fa}}, & \underline{a}_{ss,n}^{(j)} \in \mathcal{M}_n^{(j)} \\ 1 - p_d(\underline{u}_{ss,n}^{(j)}), & \underline{a}_{ss,n}^{(j)} = 0, \end{cases} \quad (12)$$

$q_{S1}(\underline{r}_{s,n}^{(j)}, \underline{u}_{ss,n}^{(j)}, \underline{r}_{ss,n}^{(j)} = 0, \underline{a}_{ss,n}^{(j)} = 0) = 1$ , and  $q_{S1}(\underline{r}_{s,n}^{(j)}, \underline{u}_{ss,n}^{(j)}, \underline{r}_{ss,n}^{(j)} = 0, \underline{a}_{ss,n}^{(j)} = m) = 0$  and  $q_{S1}(\underline{r}_{s,n}^{(j)} = 0, \underline{u}_{ss,n}^{(j)}, \underline{r}_{ss,n}^{(j)} = 1, \underline{a}_{ss,n}^{(j)}) = 0$  for the *invalid cases* ②.

The function  $q_{D1}(\underline{y}_{s,n}^{(j)}, \underline{y}_{s',n}^{(j)}, \underline{\beta}_{ss',n}^{(j)}, \underline{a}_{ss',n}^{(j)}) = q_{D1}(\underline{r}_{s,n}^{(j)}, \underline{r}_{s',n}^{(j)}, \underline{u}_{ss',n}^{(j)}, \underline{r}_{ss',n}^{(j)}, \underline{a}_{ss',n}^{(j)})$  integrating the definition of the exclusion function  $\Gamma_{\underline{a}_n^{(j)}}(\underline{r}_{s,n}^{(j)}, \underline{r}_{s',n}^{(j)}, \underline{r}_{ss',n}^{(j)})$  is given by

$$q_{D1}(\underline{r}_{s,n}^{(j)} = 1, \underline{r}_{s',n}^{(j)} = 1, \underline{u}_{ss',n}^{(j)}, \underline{r}_{ss',n}^{(j)} = 1, \underline{a}_{ss',n}^{(j)}) \triangleq \begin{cases} \frac{p_d(\underline{u}_{ss',n}^{(j)})}{\mu_{fa}}, & \underline{a}_{ss',n}^{(j)} \in \mathcal{M}_n^{(j)} \\ 1 - p_d(\underline{u}_{ss',n}^{(j)}), & \underline{a}_{ss',n}^{(j)} = 0, \end{cases} \quad (13)$$

$q_{D1}(\underline{r}_{s,n}^{(j)}, \underline{r}_{s',n}^{(j)}, \underline{u}_{ss',n}^{(j)}, \underline{r}_{ss',n}^{(j)} = 0, \underline{a}_{ss',n}^{(j)} = 0) = 1$ , and  $q_{D1}(\dots) = 0$  for  $\{\underline{r}_{s,n}^{(j)}, \underline{r}_{s',n}^{(j)}, \underline{r}_{ss',n}^{(j)}\} \in \{(0, 1, 1), (1, 0, 1), (0, 0, 1)\}$  and  $q_{D1}(\underline{r}_{s,n}^{(j)}, \underline{r}_{s',n}^{(j)}, \underline{u}_{ss',n}^{(j)}, \underline{r}_{ss',n}^{(j)} = 0, \underline{a}_{ss',n}^{(j)} = m) = 0$  represent the *invalid cases* ③.

The function  $\bar{q}_{N1}(\underline{y}_{m,n}^{(j)}, \underline{\beta}_{m,n}^{(j)}, \underline{a}_{m,n}^{(j)}) = \bar{q}_{N1}(\underline{r}_{m,n}^{(j)}, \underline{u}_{mm,n}^{(j)}, \underline{r}_{mm,n}^{(j)}, \underline{a}_{m,n}^{(j)})$  integrating the definition of the exclusion function  $\Gamma_{\underline{a}_n^{(j)}}(\underline{r}_{m,n}^{(j)}, \underline{r}_{mm,n}^{(j)})$  is given by

$$\bar{q}_{N1}(\underline{r}_{m,n}^{(j)} = 1, \underline{u}_{mm,n}^{(j)}, \underline{r}_{mm,n}^{(j)} = 1, \underline{a}_{m,n}^{(j)}) \triangleq \begin{cases} 0, & \underline{a}_{m,n}^{(j)} \in \tilde{\mathcal{D}}_n^{(j)} \\ \frac{\mu_n f_n(\underline{\mathbf{p}}_{m,\text{sfv}}^{(j)}, \underline{u}_{mm,n}^{(j)} | \mathbf{x}_n)}{\mu_{fa}}, & \underline{a}_{m,n}^{(j)} = 0, \end{cases} \quad (14)$$

$\bar{q}_{N1}(\underline{r}_{m,n}^{(j)} = 0, \underline{u}_{mm,n}^{(j)}, \underline{r}_{mm,n}^{(j)} = 0, \underline{a}_{m,n}^{(j)}) \triangleq f_D(\underline{\mathbf{p}}_{m,\text{sfv}}^{(j)}) f_D(\underline{u}_{m',n}^{(j)})$ , otherwise  $\bar{q}_{N1}(\dots) = 0$  for the *invalid cases* ④.

Finally, by inserting (10) into (1), the joint prior PDF can be rewritten as

$$\begin{aligned} & f(\mathbf{x}_{0:n}, \mathbf{y}_{0:n}, \boldsymbol{\beta}_{0:n}, \underline{\mathbf{a}}_{1:n}, \bar{\mathbf{a}}_{1:n}, \mathbf{m}_{1:n}) \\ & \propto \left( f(\mathbf{x}_0) \prod_{s=1}^{S_0} f(\mathbf{y}_{s,0}) \prod_{j'=1}^J \prod_{(s,s') \in \tilde{\mathcal{D}}_0^{(j')}} f(\boldsymbol{\beta}_{ss',0}^{(j')}) \right) \prod_{n'=1}^n f(\mathbf{x}_{n'} | \mathbf{x}_{n'-1}) \left( \left( \prod_{m'=1}^{M_n^{(j)}} \psi(\underline{a}_{00,n}^{(j)}, \bar{a}_{m',n}^{(j)}) \right) \prod_{j=1}^J q_{P1}(\boldsymbol{\beta}_{00,n}^{(j)}, \underline{a}_{00,n}^{(j)}) \right) \\ & \times \underbrace{\left( \prod_{s'=1}^{S_{n'-1}} f(\underline{\mathbf{y}}_{s',n'} | \underline{\mathbf{y}}_{s',n'-1}) \right) \left( \prod_{j'=2}^J \prod_{s'=1}^{S_{n'}^{(j')}} f^{(j)}(\underline{\mathbf{y}}_{s',n'}^{(j')} | \underline{\mathbf{y}}_{s',n'-1}^{(j'-1)}) \right)}_{\text{legacy PSFVs state transition}} \underbrace{\left( \prod_{j''=1}^J \prod_{(s,s') \in \tilde{\mathcal{D}}_{n'}^{(j'')}} f(\boldsymbol{\beta}_{ss',n'}^{(j'')} | \boldsymbol{\beta}_{ss',n'-1}^{(j'')}) \right)}_{\text{legacy PRs state transition}} \\ & \times \left( \left( \prod_{m'=1}^{M_n^{(j)}} \psi(\underline{a}_{ss,n}^{(j)}, \bar{a}_{m',n}^{(j)}) \right) \prod_{s=1}^{S_n^{(j)}} q_{S1}(\underline{\mathbf{y}}_{s,n}^{(j)}, \underline{\beta}_{ss,n}^{(j)}, \underline{a}_{ss,n}^{(j)}) \left( \prod_{m'=1}^{M_n^{(j)}} \psi(\underline{a}_{ss',n}^{(j)}, \bar{a}_{m',n}^{(j)}) \right) \right) \\ & \times \prod_{s'=1, s \neq s'}^{S_n^{(j)}} q_{D1}(\underline{\mathbf{y}}_{s,n}^{(j)}, \underline{\mathbf{y}}_{s',n}^{(j)}, \underline{\beta}_{ss',n}^{(j)}, \underline{a}_{ss',n}^{(j)}) \left( \prod_{m=1}^{M_n^{(j)}} \bar{q}_{N2}(\mathbf{x}_n, \underline{\mathbf{y}}_{m,n}^{(j)}, \underline{\beta}_{m,n}^{(j)}, \bar{a}_{m,n}^{(j)}; \mathbf{z}_n^{(j)}) \right). \end{aligned} \quad (15)$$

### B. Joint Likelihood Function

Following [2], the joint likelihood function  $f(\mathbf{z}_{1:n}|\mathbf{x}_{0:n}, \mathbf{y}_{0:n}, \boldsymbol{\beta}_{0:n}, \underline{\mathbf{a}}_{1:n}, \bar{\mathbf{a}}_{1:n}, \mathbf{m}_{1:n})$  can be written as

$$\begin{aligned} & f(\mathbf{z}_{1:n}|\mathbf{x}_{0:n}, \mathbf{y}_{0:n}, \boldsymbol{\beta}_{0:n}, \underline{\mathbf{a}}_{1:n}, \bar{\mathbf{a}}_{1:n}, \mathbf{m}_{1:n}) \\ & \propto \prod_{n'=1}^n \prod_{j=1}^J \left( q_{\text{P2}}(\mathbf{x}_n, \underline{\boldsymbol{\beta}}_{00,n}^{(j)}, \underline{\mathbf{a}}_{00,n}^{(j)}; \mathbf{z}_n^{(j)}) \prod_{s=1}^{S_{n'-1}} q_{\text{S2}}(\mathbf{x}_n, \underline{\mathbf{y}}_{s,n}^{(j)}, \underline{\boldsymbol{\beta}}_{ss,n}^{(j)}, \underline{\mathbf{a}}_{ss,n}^{(j)}; \mathbf{z}_n^{(j)}) \right. \\ & \quad \times \left. \prod_{s'=1, s' \neq s}^{S_n^{(j)}} q_{\text{D}}(\mathbf{x}_n, \underline{\mathbf{y}}_{s,n}^{(j)}, \underline{\mathbf{y}}_{s',n}^{(j)}, \underline{\boldsymbol{\beta}}_{ss',n}^{(j)}, \underline{\mathbf{a}}_{ss',n}^{(j)}; \mathbf{z}_n^{(j)}) \right) \left( \prod_{m=1}^{M_n^{(j)}} \bar{q}_{\text{N2}}(\bar{\mathbf{y}}_{m,n}^{(j)}, \bar{\boldsymbol{\beta}}_{m,n}^{(j)}, \bar{\mathbf{a}}_{m,n}^{(j)}) \right). \end{aligned} \quad (16)$$

The definitions of the functions  $q_{\text{P2}}(\cdots)$ ,  $q_{\text{S2}}(\cdots)$ ,  $q_{\text{D2}}(\cdots)$  and  $\bar{q}_{\text{N2}}(\cdots)$ , together with a summary of the functions  $q_{\text{P1}}(\cdots)$ ,  $q_{\text{S1}}(\cdots)$ ,  $q_{\text{D1}}(\cdots)$  and  $\bar{q}_{\text{N1}}(\cdots)$  are provided in the following table.

### C. Joint Posterior PDF

Assume that the measurements are observed and thus fixed. By using Bayes rule and common assumptions, the joint posterior PDF is obtained as

$$\begin{aligned} & f(\mathbf{x}_{0:n}, \mathbf{y}_{0:n}, \boldsymbol{\beta}_{0:n}, \underline{\mathbf{a}}_{1:n}, \bar{\mathbf{a}}_{1:n}, \mathbf{m}_{1:n}|\mathbf{z}_{1:n}) \\ & = \sum_{M_1'=0}^{\infty} \sum_{M_2'=0}^{\infty} \cdots \sum_{M_n'=0}^{\infty} f(\mathbf{z}_{1:n}|\mathbf{x}_{0:n}, \mathbf{y}_{0:n}, \boldsymbol{\beta}_{0:n}, \underline{\mathbf{a}}_{1:n}, \bar{\mathbf{a}}_{1:n}, \mathbf{m}_{1:n}') f(\mathbf{x}_{0:n}, \mathbf{y}_{0:n}, \boldsymbol{\beta}_{0:n}, \underline{\mathbf{a}}_{1:n}, \bar{\mathbf{a}}_{1:n}, \mathbf{m}_{1:n}'). \end{aligned} \quad (17)$$

By substituting the joint prior PDF with (15) and the joint likelihood function with (16), the joint posterior PDF can be written as

$$\begin{aligned} & f(\mathbf{x}_{0:n}, \mathbf{y}_{0:n}, \boldsymbol{\beta}_{0:n}, \underline{\mathbf{a}}_{1:n}, \bar{\mathbf{a}}_{1:n}|\mathbf{z}_{1:n}) \\ & \propto \left( f(\mathbf{x}_0) \prod_{s=1}^{S_0} f(\mathbf{y}_{s,0}) \prod_{j''=1}^J \prod_{(s,s') \in \tilde{\mathcal{D}}_0^{(j'')}} f(\boldsymbol{\beta}_{ss',0}^{(j'')}) \right) \prod_{n'=1}^n f(\mathbf{x}_{n'}|\mathbf{x}_{n'-1}) \left( \prod_{s'=1}^{S_{n'-1}} f(\underline{\mathbf{y}}_{s',n'}|\mathbf{y}_{s',n'-1}) \right) \left( \prod_{j'=2}^J \prod_{s'=1}^{S_{n'}^{(j')}} f^{(j')}(\underline{\mathbf{y}}_{s',n'}^{(j')}, |\mathbf{y}_{s',n'}^{(j'-1)}) \right) \\ & \quad \times \left( \prod_{j=1}^J f(\underline{\boldsymbol{\beta}}_{00,n'}^{(j)}|\boldsymbol{\beta}_{00,n'-1}^{(j)}) \underbrace{q_{\text{P}}(\mathbf{x}_{n'}, \underline{\boldsymbol{\beta}}_{00,n'}^{(j)}, \underline{\mathbf{a}}_{00,n'}^{(j)}; \mathbf{z}_{n'}^{(j)})}_{\triangleq q_{\text{P1}}(\cdots)q_{\text{P2}}(\cdots)} \prod_{m'=1}^{M_{n'}^{(j)}} \psi(\underline{\mathbf{a}}_{00,n'}^{(j)}, \bar{\mathbf{a}}_{m',n'}^{(j)}) \right) \\ & \quad \times \prod_{j=1}^J \left( \prod_{s=1}^{S_{n'}^{(j)}} f(\underline{\boldsymbol{\beta}}_{ss,n'}^{(j)}|\boldsymbol{\beta}_{ss,n'-1}^{(j)}) \underbrace{q_{\text{S}}(\mathbf{x}_{n'}, \underline{\mathbf{y}}_{s,n'}^{(j)}, \underline{\boldsymbol{\beta}}_{ss,n'}^{(j)}, \underline{\mathbf{a}}_{ss,n'}^{(j)}; \mathbf{z}_{n'}^{(j)})}_{\triangleq q_{\text{S1}}(\cdots)q_{\text{S2}}(\cdots)} \prod_{m'=1}^{M_{n'}^{(j)}} \psi(\underline{\mathbf{a}}_{ss,n'}^{(j)}, \bar{\mathbf{a}}_{m',n'}^{(j)}) \right) \\ & \quad \times \left( \prod_{s'=1, s' \neq s}^{S_{n'}^{(j)}} f(\underline{\boldsymbol{\beta}}_{ss',n'}^{(j)}|\boldsymbol{\beta}_{ss',n'-1}^{(j)}) \underbrace{q_{\text{D}}(\mathbf{x}_{n'}, \underline{\mathbf{y}}_{s,n'}^{(j)}, \underline{\mathbf{y}}_{s',n'}^{(j)}, \underline{\boldsymbol{\beta}}_{ss',n'}^{(j)}, \underline{\mathbf{a}}_{ss',n'}^{(j)}; \mathbf{z}_{n'}^{(j)})}_{\triangleq q_{\text{D1}}(\cdots)q_{\text{D2}}(\cdots)} \prod_{m'=1}^{M_{n'}^{(j)}} \psi(\underline{\mathbf{a}}_{ss',n'}^{(j)}, \bar{\mathbf{a}}_{m',n'}^{(j)}) \right) \\ & \quad \times \left( \prod_{m=1}^{M_{n'}^{(j)}} \bar{q}_{\text{N}}(\mathbf{x}_{n'}, \bar{\mathbf{y}}_{m,n'}^{(j)}, \bar{\boldsymbol{\beta}}_{m,n'}^{(j)}, \bar{\mathbf{a}}_{m,n'}^{(j)}; \mathbf{z}_{n'}^{(j)}) \right). \end{aligned} \quad (18)$$

| Summary of exclusion functions and pseudo LHF's                                                                                                                                                                                                                                                                                                                                                                                                                                                                                                                                                                                                                                                                                                    |                                                                                                 |                                                    |                                                                                                                                                                          |                                                                                                                                                                                                                 |
|----------------------------------------------------------------------------------------------------------------------------------------------------------------------------------------------------------------------------------------------------------------------------------------------------------------------------------------------------------------------------------------------------------------------------------------------------------------------------------------------------------------------------------------------------------------------------------------------------------------------------------------------------------------------------------------------------------------------------------------------------|-------------------------------------------------------------------------------------------------|----------------------------------------------------|--------------------------------------------------------------------------------------------------------------------------------------------------------------------------|-----------------------------------------------------------------------------------------------------------------------------------------------------------------------------------------------------------------|
| cases                                                                                                                                                                                                                                                                                                                                                                                                                                                                                                                                                                                                                                                                                                                                              | exclusion function                                                                              | pseudo LHF part1                                   | pseudo LHF part2                                                                                                                                                         | pseudo LHF                                                                                                                                                                                                      |
| For PAs and LoSs PRs<br>i.e., $(s, s') = (0, 0)$<br>$r_{00,n}^{(j)} = 1, \underline{q}_{00,n}^{(j)} \in \mathcal{M}_n^{(j)}$<br>$r_{00,n}^{(j)} = 1, \underline{q}_{00,n}^{(j)} = 0$<br>$r_{00,n}^{(j)} = 0, \underline{q}_{00,n}^{(j)} = 0$<br>$r_{00,n}^{(j)} = 0, \underline{q}_{00,n}^{(j)} \in \mathcal{M}_n^{(j)}$                                                                                                                                                                                                                                                                                                                                                                                                                           | $\Gamma_{\underline{q}_n^{(j)}}(r_{00,n}^{(j)})$                                                | $\underline{q}_{P1}(\cdots)$                       | $\underline{q}_{P2}(\cdots)$                                                                                                                                             | $\underline{q}_P(\cdots) \triangleq \underline{q}_{P1}(\cdots)\underline{q}_{P2}(\cdots)$                                                                                                                       |
|                                                                                                                                                                                                                                                                                                                                                                                                                                                                                                                                                                                                                                                                                                                                                    | 1                                                                                               | $\frac{Pd(\underline{u}_{00,n}^{(j)})}{\mu_{fa}}$  | $\frac{f_P(\mathbf{z}_{m,n}^{(j)} \mathbf{p}_n, \underline{u}_{00,n}^{(j)})}{f_{fa}(\mathbf{z}_{m,n}^{(j)})}$                                                            | $\frac{f_P(\mathbf{z}_{m,n}^{(j)} \mathbf{p}_n, \underline{u}_{00,n}^{(j)})Pd(\underline{u}_{00,n}^{(j)})}{\mu_{fa}f_{fa}(\mathbf{z}_{m,n}^{(j)})}$                                                             |
|                                                                                                                                                                                                                                                                                                                                                                                                                                                                                                                                                                                                                                                                                                                                                    | 1                                                                                               | $1 - Pd(\underline{u}_{00,n}^{(j)})$               | 1                                                                                                                                                                        | $1 - Pd(\underline{u}_{00,n}^{(j)})$                                                                                                                                                                            |
|                                                                                                                                                                                                                                                                                                                                                                                                                                                                                                                                                                                                                                                                                                                                                    | 1                                                                                               | 1                                                  | 1                                                                                                                                                                        | 1                                                                                                                                                                                                               |
|                                                                                                                                                                                                                                                                                                                                                                                                                                                                                                                                                                                                                                                                                                                                                    | 0                                                                                               | 0                                                  | 0                                                                                                                                                                        | 0                                                                                                                                                                                                               |
| For legacy PSFVs and single-bounce PRs<br>i.e., $s = s' \wedge (s, s') \neq (0, 0)$<br>$r_{ss,n}^{(j)} = 1, \underline{r}_{ss,n}^{(j)} = 1, \underline{q}_{ss,n}^{(j)} \in \mathcal{M}_n^{(j)}$<br>$r_{ss,n}^{(j)} = 1, \underline{r}_{ss,n}^{(j)} = 1, \underline{q}_{ss,n}^{(j)} = 0$<br>$r_{ss,n}^{(j)}, \underline{r}_{ss,n}^{(j)} = 0, \underline{q}_{ss,n}^{(j)} = 0$<br>$r_{ss,n}^{(j)}, \underline{r}_{ss,n}^{(j)} = 0, \underline{q}_{ss,n}^{(j)} \in \mathcal{M}_n^{(j)}$<br>$r_{ss,n} = 0, \underline{r}_{ss,n} = 1, \underline{q}_{ss,n} \in \mathcal{M}_{0,n}^{(j)}$                                                                                                                                                                  | $\Gamma_{\underline{q}_n^{(j)}}(r_{ss,n}^{(j)}, \underline{r}_{ss,n}^{(j)})$                    | $\underline{q}_{S1}(\cdots)$                       | $\underline{q}_{S2}(\cdots)$                                                                                                                                             | $\underline{q}_S(\cdots) \triangleq \underline{q}_{S1}(\cdots)\underline{q}_{S2}(\cdots)$                                                                                                                       |
|                                                                                                                                                                                                                                                                                                                                                                                                                                                                                                                                                                                                                                                                                                                                                    | 1                                                                                               | $\frac{Pd(\underline{u}_{ss,n}^{(j)})}{\mu_{fa}}$  | $\frac{f_S(\mathbf{z}_{m,n}^{(j)} \mathbf{p}_n, \underline{r}_{ss,n}^{(j)}, \underline{u}_{ss,n}^{(j)})}{f_{fa}(\mathbf{z}_{m,n}^{(j)})}$                                | $\frac{f_S(\mathbf{z}_{m,n}^{(j)} \mathbf{p}_n, \underline{r}_{ss,n}^{(j)}, \underline{u}_{ss,n}^{(j)})Pd(\underline{u}_{ss,n}^{(j)})}{\mu_{fa}f_{fa}(\mathbf{z}_{m,n}^{(j)})}$                                 |
|                                                                                                                                                                                                                                                                                                                                                                                                                                                                                                                                                                                                                                                                                                                                                    | 1                                                                                               | $1 - Pd(\underline{u}_{ss,n}^{(j)})$               | 1                                                                                                                                                                        | $1 - Pd(\underline{u}_{ss,n}^{(j)})$                                                                                                                                                                            |
|                                                                                                                                                                                                                                                                                                                                                                                                                                                                                                                                                                                                                                                                                                                                                    | 1                                                                                               | 1                                                  | 1                                                                                                                                                                        | 1                                                                                                                                                                                                               |
|                                                                                                                                                                                                                                                                                                                                                                                                                                                                                                                                                                                                                                                                                                                                                    | 0                                                                                               | 0                                                  | 0                                                                                                                                                                        | 0                                                                                                                                                                                                               |
| For legacy PSFVs and double-bounce PRs<br>i.e., $s \neq s' \wedge (s, s') \neq (0, 0)$<br>$r_{ss',n}^{(j)} = 1, \underline{r}_{ss',n}^{(j)} = 1, \underline{q}_{ss',n}^{(j)} \in \mathcal{M}_n^{(j)}$<br>$r_{ss',n}^{(j)} = 1, \underline{r}_{ss',n}^{(j)} = 1, \underline{q}_{ss',n}^{(j)} = 0$<br>$\forall (r_{ss',n}^{(j)}, \underline{r}_{ss',n}^{(j)})$ , $\underline{r}_{ss',n}^{(j)} = 0, \underline{q}_{ss',n}^{(j)} = 0$<br>$\forall (r_{ss',n}^{(j)}, \underline{r}_{ss',n}^{(j)})$ , $\underline{r}_{ss',n}^{(j)} = 0, \underline{q}_{ss',n}^{(j)} \in \mathcal{M}_n^{(j)}$<br>$(r_{ss',n}^{(j)} = 0) \vee (\underline{r}_{ss',n}^{(j)} = 0), \underline{r}_{ss',n}^{(j)} = 1, \underline{q}_{ss',n}^{(j)} \in \mathcal{M}_{0,n}^{(j)}$ | $\Gamma_{\underline{q}_n^{(j)}}(r_{ss',n}^{(j)}, \underline{r}_{ss',n}^{(j)}, r_{ss',n}^{(j)})$ | $\underline{q}_{D1}(\cdots)$                       | $\underline{q}_{D2}(\cdots)$                                                                                                                                             | $\underline{q}_D(\cdots) \triangleq \underline{q}_{D1}(\cdots)\underline{q}_{D2}(\cdots)$                                                                                                                       |
|                                                                                                                                                                                                                                                                                                                                                                                                                                                                                                                                                                                                                                                                                                                                                    | 1                                                                                               | $\frac{Pd(\underline{u}_{ss',n}^{(j)})}{\mu_{fa}}$ | $\frac{f_D(\mathbf{z}_{m,n}^{(j)} \mathbf{p}_n, \underline{r}_{ss',n}^{(j)}, \underline{r}_{ss',n}^{(j)}, \underline{u}_{ss',n}^{(j)})}{f_{fa}(\mathbf{z}_{m,n}^{(j)})}$ | $\frac{f_D(\mathbf{z}_{m,n}^{(j)} \mathbf{p}_n, \underline{r}_{ss',n}^{(j)}, \underline{r}_{ss',n}^{(j)}, \underline{u}_{ss',n}^{(j)})Pd(\underline{u}_{ss',n}^{(j)})}{\mu_{fa}f_{fa}(\mathbf{z}_{m,n}^{(j)})}$ |
|                                                                                                                                                                                                                                                                                                                                                                                                                                                                                                                                                                                                                                                                                                                                                    | 1                                                                                               | $1 - Pd(\underline{u}_{ss',n}^{(j)})$              | 1                                                                                                                                                                        | $1 - Pd(\underline{u}_{ss',n}^{(j)})$                                                                                                                                                                           |
|                                                                                                                                                                                                                                                                                                                                                                                                                                                                                                                                                                                                                                                                                                                                                    | 1                                                                                               | 1                                                  | 1                                                                                                                                                                        | 1                                                                                                                                                                                                               |
|                                                                                                                                                                                                                                                                                                                                                                                                                                                                                                                                                                                                                                                                                                                                                    | 0                                                                                               | 0                                                  | 0                                                                                                                                                                        | 0                                                                                                                                                                                                               |

| Summary of exclusion functions and pseudo LHF's                                                              |                                                                             |                                                                                                                 |                                                                                                                                                                                            |                                                                                                                                                                                                                                                                                                  |
|--------------------------------------------------------------------------------------------------------------|-----------------------------------------------------------------------------|-----------------------------------------------------------------------------------------------------------------|--------------------------------------------------------------------------------------------------------------------------------------------------------------------------------------------|--------------------------------------------------------------------------------------------------------------------------------------------------------------------------------------------------------------------------------------------------------------------------------------------------|
| cases                                                                                                        | exclusion function                                                          | pseudo LHF part1                                                                                                | pseudo LHF part2                                                                                                                                                                           | pseudo LHF                                                                                                                                                                                                                                                                                       |
| For new PSFV's and new PRs                                                                                   | $\Gamma_{\underline{q}_n^{(j)}}(\bar{r}_{m,n}^{(j)}, \bar{r}_{mm,n}^{(j)})$ | $\underline{q}_{N1}(\dots)$                                                                                     | $\underline{q}_{N2}(\dots)$                                                                                                                                                                | $\underline{q}_N(\dots) \triangleq \underline{q}_{N1}(\dots)\underline{q}_{N2}(\dots)$                                                                                                                                                                                                           |
| $\bar{r}_{m,n}^{(j)} = 1, \bar{r}_{mm,n}^{(j)} = 1, \underline{q}_{ss',n}^{(j)} = 0$                         | 1                                                                           | $\frac{\mu_n f_n(\bar{\mathbf{p}}_{m,\text{sfv}}^{(j)}, \bar{u}_{mm,n}^{(j)}   \mathbf{x}_n)}{\mu_{\text{fa}}}$ | $\frac{f(z_{m,n}^{(j)}   \mathbf{p}_n, \bar{\mathbf{p}}_{m,\text{sfv}}^{(j)}, \underline{\mathbf{p}}_{\mathcal{I},\text{sfv}}^{(j)}, \bar{u}_{mm,n}^{(j)})}{f_{\text{fa}}(z_{m,n}^{(j)})}$ | $\frac{f(z_{m,n}^{(j)}   \mathbf{p}_n, \bar{\mathbf{p}}_{m,\text{sfv}}^{(j)}, \underline{\mathbf{p}}_{\mathcal{V},\text{sfv}}^{(j)}, \bar{u}_{mm,n}^{(j)}) \mu_n f_n(\bar{\mathbf{p}}_{m,\text{sfv}}^{(j)}, \bar{u}_{mm,n}^{(j)}   \mathbf{x}_n)}{\mu_{\text{fa}} f_{\text{fa}}(z_{m,n}^{(j)})}$ |
| $\bar{r}_{m,n}^{(j)} = 0, \bar{r}_{mm,n}^{(j)} = 0, \underline{q}_{ss',n}^{(j)} \in \mathcal{M}_{0,n}^{(j)}$ | 1                                                                           | $f_{\text{D}}(\bar{\mathbf{p}}_{m',\text{sfv}}^{(j)}) f_{\text{D}}(\bar{u}_{m'm',n}^{(j)})$                     | 1                                                                                                                                                                                          | $f_{\text{D}}(\bar{\mathbf{p}}_{m',\text{sfv}}^{(j)}) f_{\text{D}}(\bar{u}_{m'm',n}^{(j)})$                                                                                                                                                                                                      |
| otherwise                                                                                                    | 0                                                                           | 0                                                                                                               | 0                                                                                                                                                                                          | 0                                                                                                                                                                                                                                                                                                |

## II. SUM-PRODUCT ALGORITHM

Due to the loops inside the factor graph, we specify the following orders for message computation: (i) messages are sent forward both in time from  $n-1$  to  $n$  and serially from PA  $j-1$  to  $j$ ; (ii) iterative message passing is only performed for probabilistic data association (DA), i.e., message passing iteration is performed only once in the loops connecting different PSFVs; (iii) messages are only sent from the agent state variable node to the new PSFV state variable node, not vice versa. Combining the specified orders with the generic SPA rules for calculating messages and beliefs yields the following calculations at each time  $n$  and each PA  $j$ :

### A. Prediction

1) *Transition from Time  $n-1$  to  $n$ :* First, a prediction step from time  $n-1$  to  $n$  is performed for the agent state, all legacy PSFV states and PR states. The predicted messages for the agent state are given by

$$\alpha(\mathbf{x}_n) = \int f(\mathbf{x}_n | \mathbf{x}_{n-1}) \tilde{f}(\mathbf{x}_{n-1}) d\mathbf{x}_{n-1}. \quad (19)$$

For all the legacy PSFVs  $s \in \mathcal{S}_{n-1}$ , the predicted messages are given by

$$\alpha(\underline{\mathbf{p}}_{s,\text{sfv}}, \underline{r}_{s,n}) = \sum_{r_{s,n-1} \in \{0,1\}} \int f(\underline{\mathbf{p}}_{s,\text{sfv}}, \underline{r}_{s,n} | \mathbf{p}_{s,\text{sfv}}, r_{s,n-1}) \tilde{f}(\mathbf{p}_{s,\text{sfv}}, r_{s,n-1}) d\mathbf{p}_{s,\text{sfv}}. \quad (20)$$

By inserting (9) and (10) in [1], we further obtain

$$\alpha(\underline{\mathbf{p}}_{s,\text{sfv}}, \underline{r}_{s,n} = 1) = p_s \int f(\underline{\mathbf{p}}_{s,\text{sfv}} | \mathbf{p}_{s,\text{sfv}}) \tilde{f}(\mathbf{p}_{s,\text{sfv}}, 1) d\mathbf{p}_{s,\text{sfv}} \quad (21)$$

for existing PSFVs and  $\alpha(\underline{\mathbf{p}}_{s,\text{sfv}}, \underline{r}_{s,n} = 0) = \alpha_{s,n} f_D(\underline{\mathbf{p}}_{s,\text{sfv}})$  for nonexistent PSFVs with

$$\alpha_{s,n} = (1 - p_s) \int \tilde{f}(\mathbf{p}_{s,\text{sfv}}, 1) d\mathbf{p}_{s,\text{sfv}} + \tilde{f}_{s,n-1}. \quad (22)$$

and  $\tilde{f}_{s,n-1} = \int \tilde{f}(\mathbf{p}_{s,\text{sfv}}, 0) d\mathbf{p}_{s,\text{sfv}}$  approximating the nonexistent probability of legacy PSFV  $s$  at the previous time. Similarly, the predicted messages  $\alpha(\underline{\beta}_{ss',n}^{(j)}) = \alpha(\underline{u}_{ss',n}^{(j)}, \underline{r}_{ss',n}^{(j)})$  for legacy PRs are obtained as

$$\alpha(\underline{u}_{ss',n}^{(j)}, \underline{r}_{ss',n}^{(j)}) = \sum_{r_{ss',n-1}^{(j)} \in \{0,1\}} \int f(\underline{u}_{ss',n}^{(j)}, \underline{r}_{ss',n}^{(j)} | u_{ss',n-1}^{(j)}, r_{ss',n-1}^{(j)}) \tilde{f}(u_{ss',n-1}^{(j)}, r_{ss',n-1}^{(j)}) du_{ss',n-1}^{(j)}. \quad (23)$$

By inserting (13) and (14) in [1], we further obtain

$$\alpha(\underline{u}_{ss',n}^{(j)}, \underline{r}_{ss',n}^{(j)} = 1) = p_s \int f(\underline{u}_{ss',n}^{(j)} | u_{ss',n-1}^{(j)}) \tilde{f}(u_{ss',n-1}^{(j)}, 1) du_{ss',n-1}^{(j)} \quad (24)$$

for existing PRs and  $\alpha(\underline{u}_{ss',n}^{(j)}, \underline{r}_{ss',n}^{(j)} = 0) = \alpha_{ss',n}^{(j)} f_D(\underline{u}_{ss',n}^{(j)})$  for nonexistent PRs with

$$\alpha_{ss',n}^{(j)} = (1 - p_s) \int \tilde{f}(u_{ss',n-1}^{(j)}, 1) du_{ss',n-1}^{(j)} + \tilde{f}_{ss',n-1}^{(j)} \quad (25)$$

and  $\tilde{f}_{ss',n-1}^{(j)} = \int \tilde{f}(u_{ss',n-1}^{(j)}, 0) du_{ss',n-1}^{(j)}$  approximating the nonexistent probability of legacy PR  $(s, s')$  at the previous time  $n-1$ . The beliefs of the agent state  $\tilde{f}(\mathbf{x}_{n-1})$ , of the PSFV states  $\tilde{f}(\mathbf{p}_{s,\text{sfv}}, r_{s,n-1})$ , and of the PR states  $\tilde{f}(u_{ss',n-1}^{(j)}, r_{ss',n-1}^{(j)})$  are obtained at time  $n-1$ .

2) *Transition from PA  $j-1$  to  $j$ :* For  $j > 1$ , the predicted messages  $\alpha(\underline{\mathbf{p}}_{s,\text{sfv}}^{(j)}, \underline{r}_{s,n}^{(j)})$  for the former legacy PSFVs  $s \in \mathcal{S}_n^{(j-1)}$  and the predicted messages  $\alpha(\underline{\mathbf{p}}_{\mathcal{S}_n^{(j-1)}+m,\text{sfv}}^{(j)}, \underline{r}_{\mathcal{S}_n^{(j-1)}+m,n}^{(j)})$  for the former new PSFVs  $m \in \mathcal{M}_n^{(j-1)}$  are inline with [2].

### B. Sequential PA Update

1) *Measurement Evaluation for the LoS Path:* The messages  $\omega(\underline{a}_{00,n}^{(j)})$  propagate from the  $j$ th PA related factor node  $\underline{q}_P(\mathbf{x}_n, \underline{\beta}_{00,n}^{(j)}, \underline{a}_{00,n}^{(j)}; \mathbf{z}_n^{(j)})$  to the feature-oriented association variable nodes  $\underline{a}_{00,n}^{(j)}$  are given by

$$\begin{aligned}
\omega(\underline{a}_{00,n}^{(j)}) &= \sum_{r_{00,n}^{(j)} \in \{0,1\}} \iint \alpha(\mathbf{x}_n) \alpha(\underline{u}_{00,n}^{(j)}, r_{00,n}^{(j)}) \underline{q}_P(\mathbf{x}_n, \underline{u}_{00,n}^{(j)}, r_{00,n}^{(j)}, \underline{a}_{00,n}^{(j)}; \mathbf{z}_n^{(j)}) d\mathbf{x}_n du_{00,n}^{(j)} \\
&= \iint \alpha(\mathbf{x}_n) \alpha(\underline{u}_{00,n}^{(j)}, 1) \underline{q}_P(\mathbf{x}_n, \underline{u}_{00,n}^{(j)}, 1, \underline{a}_{00,n}^{(j)}; \mathbf{z}_n^{(j)}) d\mathbf{x}_n du_{00,n}^{(j)} \\
&\quad + 1(\underline{a}_{00,n}^{(j)}) \iint \alpha(\mathbf{x}_n) \alpha(\underline{u}_{00,n}^{(j)}, 0) d\mathbf{x}_n du_{00,n}^{(j)} \\
&= \iint \alpha(\mathbf{x}_n) \alpha(\underline{u}_{00,n}^{(j)}, 1) \underline{q}_P(\mathbf{x}_n, \underline{u}_{00,n}^{(j)}, 1, \underline{a}_{00,n}^{(j)}; \mathbf{z}_n^{(j)}) d\mathbf{x}_n du_{00,n}^{(j)} + 1(\underline{a}_{00,n}^{(j)}) \alpha_{00,n}^{(j)}. \tag{26}
\end{aligned}$$

#### 2) Measurement Evaluation for Legacy PSFVs:

a) *Single-bounce propagation path:* For  $s = s'$ , the messages  $\omega(\underline{a}_{ss,n}^{(j)})$  propagate from the single-bounce PR related factor node  $\underline{q}_S(\mathbf{x}_n, \underline{\mathbf{y}}_{s,n}^{(j)}, \underline{\beta}_{ss,n}^{(j)}, \underline{a}_{ss,n}^{(j)}; \mathbf{z}_n^{(j)})$  to the feature-oriented association variable nodes  $\underline{a}_{ss,n}^{(j)}$  are given by

$$\begin{aligned}
\omega(\underline{a}_{ss,n}^{(j)}) &= \sum_{r_{ss,n}^{(j)} \in \{0,1\}} \sum_{r_{s,n}^{(j)} \in \{0,1\}} \iiint \alpha(\mathbf{x}_n) \alpha(\underline{\mathbf{p}}_{s,\text{sfv}}^{(j)}, r_{s,n}^{(j)}) \\
&\quad \times \alpha(\underline{u}_{ss,n}^{(j)}, r_{ss,n}^{(j)}) \underline{q}_S(\mathbf{x}_n, \underline{\mathbf{p}}_{s,\text{sfv}}^{(j)}, r_{s,n}^{(j)}, \underline{u}_{ss,n}^{(j)}, r_{ss,n}^{(j)}, \underline{a}_{ss,n}^{(j)}; \mathbf{z}_n^{(j)}) d\mathbf{x}_n d\underline{\mathbf{p}}_{s,\text{sfv}}^{(j)} du_{ss,n}^{(j)} \\
&= \iiint \alpha(\mathbf{x}_n) \alpha(\underline{\mathbf{p}}_{s,\text{sfv}}^{(j)}, 1) \alpha(\underline{u}_{ss,n}^{(j)}, 1) \underline{q}_S(\mathbf{x}_n, \underline{\mathbf{p}}_{s,\text{sfv}}^{(j)}, 1, \underline{u}_{ss,n}^{(j)}, 1, \underline{a}_{ss,n}^{(j)}; \mathbf{z}_n^{(j)}) d\mathbf{x}_n d\underline{\mathbf{p}}_{s,\text{sfv}}^{(j)} du_{ss,n}^{(j)} \\
&\quad + 1(\underline{a}_{ss,n}^{(j)}) \alpha_{ss,n}^{(j)} \underbrace{\left( \alpha_{s,n}^{(j)} + \int \alpha(\underline{\mathbf{p}}_{s,\text{sfv}}^{(j)}, 1) d\underline{\mathbf{p}}_{s,\text{sfv}}^{(j)} \right)}_{=1} \\
&= \iiint \alpha(\mathbf{x}_n) \alpha(\underline{\mathbf{p}}_{s,\text{sfv}}^{(j)}, 1) \alpha(\underline{u}_{ss,n}^{(j)}, 1) \underline{q}_S(\mathbf{x}_n, \underline{\mathbf{p}}_{s,\text{sfv}}^{(j)}, 1, \underline{u}_{ss,n}^{(j)}, 1, \underline{a}_{ss,n}^{(j)}; \mathbf{z}_n^{(j)}) d\mathbf{x}_n d\underline{\mathbf{p}}_{s,\text{sfv}}^{(j)} du_{ss,n}^{(j)} \\
&\quad + 1(\underline{a}_{ss,n}^{(j)}) \alpha_{ss,n}^{(j)}. \tag{27}
\end{aligned}$$

b) *Double-bounce propagation path:* For  $s \neq s'$ , the messages  $\omega(\underline{a}_{ss',n}^{(j)})$  propagate from the double-bounce PR related factor node  $\underline{q}_D(\mathbf{x}_n, \underline{\mathbf{y}}_{s,n}^{(j)}, \underline{\mathbf{y}}_{s',n}^{(j)}, \underline{\mathbf{u}}_{ss',n}^{(j)}, \underline{a}_{ss',n}^{(j)}; \mathbf{z}_n^{(j)})$  to the feature-oriented association variable nodes  $\underline{a}_{ss',n}^{(j)}$  are

given by

$$\begin{aligned}
& \omega(\underline{a}_{ss',n}^{(j)}) \\
&= \sum_{r_{ss,n}^{(j)} \in \{0,1\}} \sum_{r_{s,n}^{(j)} \in \{0,1\}} \sum_{r_{s',n}^{(j)} \in \{0,1\}} \iiint \alpha(\mathbf{x}_n) \alpha(\underline{\mathbf{p}}_{s,\text{sfv}}^{(j)}, r_{s,n}^{(j)}) \alpha(\underline{\mathbf{p}}_{s',\text{sfv}}^{(j)}, r_{s',n}^{(j)}) \alpha(\underline{\mathbf{u}}_{ss',n}^{(j)}, r_{ss,n}^{(j)}) \\
&\quad \times q_D(\mathbf{x}_n, \underline{\mathbf{p}}_{s,\text{sfv}}^{(j)}, r_{s,n}^{(j)}, \underline{\mathbf{p}}_{s',\text{sfv}}^{(j)}, r_{s',n}^{(j)}, \underline{\mathbf{u}}_{ss',n}^{(j)}, r_{ss,n}^{(j)}, \underline{\mathbf{a}}_{ss',n}^{(j)}; \mathbf{z}_n^{(j)}) d\mathbf{x}_n d\underline{\mathbf{p}}_{s,\text{sfv}}^{(j)} d\underline{\mathbf{p}}_{s',\text{sfv}}^{(j)} d\underline{\mathbf{u}}_{ss',n}^{(j)} \\
&= \iiint \alpha(\mathbf{x}_n) \alpha(\underline{\mathbf{p}}_{s,\text{sfv}}^{(j)}, 1) \alpha(\underline{\mathbf{p}}_{s',\text{sfv}}^{(j)}, 1) \alpha(\underline{\mathbf{u}}_{ss',n}^{(j)}, 1) q_D(\mathbf{x}_n, \underline{\mathbf{p}}_{s,\text{sfv}}^{(j)}, 1, \underline{\mathbf{p}}_{s',\text{sfv}}^{(j)}, 1, \underline{\mathbf{u}}_{ss',n}^{(j)}, 1, \underline{\mathbf{a}}_{ss',n}^{(j)}; \mathbf{z}_n^{(j)}) \\
&\quad \times d\mathbf{x}_n d\underline{\mathbf{p}}_{s,\text{sfv}}^{(j)} d\underline{\mathbf{p}}_{s',\text{sfv}}^{(j)} d\underline{\mathbf{u}}_{ss',n}^{(j)} + 1(\underline{\mathbf{a}}_{ss',n}^{(j)}) \alpha_{ss',n}^{(j)} \alpha_{s',n}^{(j)} \underbrace{\left( \alpha_{s,n}^{(j)} + \int \alpha(\underline{\mathbf{p}}_{s,\text{sfv}}^{(j)}, 1) d\underline{\mathbf{p}}_{s,\text{sfv}}^{(j)} \right)}_{=1} \\
&\quad + 1(\underline{\mathbf{a}}_{ss',n}^{(j)}) \alpha_{ss',n}^{(j)} \underbrace{\left( \alpha_{s,n}^{(j)} + \int \alpha(\underline{\mathbf{p}}_{s,\text{sfv}}^{(j)}, 1) d\underline{\mathbf{p}}_{s,\text{sfv}}^{(j)} \right)}_{=1} \int \alpha(\underline{\mathbf{p}}_{s',\text{sfv}}^{(j)}, 1) d\underline{\mathbf{p}}_{s',\text{sfv}}^{(j)} \\
&= \iiint \alpha(\mathbf{x}_n) \alpha(\underline{\mathbf{p}}_{s,\text{sfv}}^{(j)}, 1) \alpha(\underline{\mathbf{p}}_{s',\text{sfv}}^{(j)}, 1) \alpha(\underline{\mathbf{u}}_{ss',n}^{(j)}, 1) q_D(\mathbf{x}_n, \underline{\mathbf{p}}_{s,\text{sfv}}^{(j)}, 1, \underline{\mathbf{p}}_{s',\text{sfv}}^{(j)}, 1, \underline{\mathbf{u}}_{ss',n}^{(j)}, 1, \underline{\mathbf{a}}_{ss',n}^{(j)}; \mathbf{z}_n^{(j)}) \\
&\quad \times d\mathbf{x}_n d\underline{\mathbf{p}}_{s,\text{sfv}}^{(j)} d\underline{\mathbf{p}}_{s',\text{sfv}}^{(j)} d\underline{\mathbf{u}}_{ss',n}^{(j)} + 1(\underline{\mathbf{a}}_{ss',n}^{(j)}) \alpha_{ss',n}^{(j)} \underbrace{\left( \alpha_{s',n}^{(j)} + \int \alpha(\underline{\mathbf{p}}_{s',\text{sfv}}^{(j)}, 1) d\underline{\mathbf{p}}_{s',\text{sfv}}^{(j)} \right)}_{=1}. \tag{28}
\end{aligned}$$

Finally, we obtain

$$\begin{aligned}
\omega(\underline{\mathbf{a}}_{ss',n}^{(j)}) &= 1(\underline{\mathbf{a}}_{ss',n}^{(j)}) \alpha_{ss',n}^{(j)} + \iiint \alpha(\mathbf{x}_n) \alpha(\underline{\mathbf{p}}_{s,\text{sfv}}^{(j)}, 1) \alpha(\underline{\mathbf{p}}_{s',\text{sfv}}^{(j)}, 1) \alpha(\underline{\mathbf{u}}_{ss',n}^{(j)}, 1) \\
&\quad \times q_D(\mathbf{x}_n, \underline{\mathbf{p}}_{s,\text{sfv}}^{(j)}, 1, \underline{\mathbf{p}}_{s',\text{sfv}}^{(j)}, 1, \underline{\mathbf{u}}_{ss',n}^{(j)}, 1, \underline{\mathbf{a}}_{ss',n}^{(j)}; \mathbf{z}_n^{(j)}) d\mathbf{x}_n d\underline{\mathbf{p}}_{s,\text{sfv}}^{(j)} d\underline{\mathbf{p}}_{s',\text{sfv}}^{(j)} d\underline{\mathbf{u}}_{ss',n}^{(j)}. \tag{29}
\end{aligned}$$

3) *Measurement Evaluation for New PSFVs:* For PA  $j$ , the messages  $\xi(\bar{\mathbf{a}}_{m,n}^{(j)})$  sent from the new PSFV and new PR related factor node  $\bar{q}_N(\mathbf{x}_n, \bar{\mathbf{y}}_{m,n}^{(j)}, \bar{\boldsymbol{\beta}}_{m,n}^{(j)}, \bar{\mathbf{a}}_{m,n}^{(j)}; \mathbf{z}_n^{(j)})$  to the measurement-oriented association variable nodes  $\bar{\mathbf{a}}_{m,n}^{(j)}$  are given by

$$\xi(\bar{\mathbf{a}}_{m,n}^{(j)}) = \sum_{\bar{\mathbf{r}}_{m,n}^{(j)} \in \{0,1\}} \sum_{\bar{\mathbf{r}}_{mm,n}^{(j)} \in \{0,1\}} \iiint \alpha(\mathbf{x}_n) \bar{q}_N(\mathbf{x}_n, \bar{\mathbf{p}}_{m,\text{sfv}}^{(j)}, \bar{\mathbf{r}}_{m,n}^{(j)}, \bar{\mathbf{u}}_{mm,n}^{(j)}, \bar{\mathbf{r}}_{mm,n}^{(j)}, \bar{\mathbf{a}}_{m,n}^{(j)}; \mathbf{z}_n^{(j)}) d\mathbf{x}_n d\bar{\mathbf{p}}_{m,\text{sfv}}^{(j)} d\bar{\mathbf{u}}_{mm,n}^{(j)}. \tag{30}$$

Specifically,  $\xi(\bar{\mathbf{a}}_{m,n}^{(j)}) = 1$  for  $\bar{\mathbf{a}}_{m,n}^{(j)} \in \tilde{\mathcal{D}}_n^{(j)}$ , and for  $\bar{\mathbf{a}}_{m,n}^{(j)} = 0$ ,

$$\xi(\bar{\mathbf{a}}_{m,n}^{(j)}) = \frac{\mu_n}{\mu_{\text{fa}} f_{\text{fa}}(\mathbf{z}_{m,n}^{(j)})} \iiint \alpha(\mathbf{x}_n) f_n(\bar{\mathbf{p}}_{m,\text{sfv}}^{(j)}, \bar{\mathbf{u}}_{mm,n}^{(j)} | \mathbf{x}_n) f(\mathbf{z}_{m,n}^{(j)} | \mathbf{p}_n, \bar{\mathbf{p}}_{m,\text{sfv}}^{(j)}, \bar{\mathbf{u}}_{mm,n}^{(j)}) d\mathbf{x}_n d\bar{\mathbf{p}}_{m,\text{sfv}}^{(j)} d\bar{\mathbf{u}}_{mm,n}^{(j)} + 1. \tag{31}$$

4) *Iterative Data Association:* With the messages  $\omega(\underline{\mathbf{a}}_{ss',n}^{(j)})$  and  $\xi(\bar{\mathbf{a}}_{m,n}^{(j)})$ , the probabilistic DA messages  $\eta(\underline{\mathbf{a}}_{ss',n}^{(j)})$  and  $\varsigma(\bar{\mathbf{a}}_{m,n}^{(j)})$  are obtained using loopy belief propagation (BP) according to [2], [3].

5) *Measurement Update for Agent:* For the update of agent state  $\mathbf{x}_n$ , only the messages from legacy PSFVs are used.

a) *LoS propagation path:* The messages  $\gamma_{00}^{(j)}(\mathbf{x}_n)$  sent from the factor node  $q_P(\mathbf{x}_n, \underline{\boldsymbol{\beta}}_{00,n}^{(j)}, \underline{\mathbf{a}}_{00,n}^{(j)}; \mathbf{z}_n^{(j)})$  to the agent variable node  $\mathbf{x}_n$  are obtained as

$$\gamma_{00}^{(j)}(\mathbf{x}_n) = \sum_{\underline{\mathbf{a}}_{00,n}^{(j)} \in \mathcal{M}_{0,n}^{(j)}} \eta(\underline{\mathbf{a}}_{00,n}^{(j)}) \int \alpha(\underline{\mathbf{u}}_{00,n}^{(j)}, 1) q_P(\mathbf{x}_n, \underline{\mathbf{u}}_{00,n}^{(j)}, 1, \underline{\mathbf{a}}_{00,n}^{(j)}; \mathbf{z}_n^{(j)}) d\underline{\mathbf{u}}_{00,n}^{(j)} + \eta(\underline{\mathbf{a}}_{00,n}^{(j)} = 0) \alpha_{00,n}^{(j)} \tag{32}$$

with  $\mathcal{M}_{0,n}^{(j)} \triangleq \{0, \mathcal{M}_n^{(j)}\}$ .

b) *Single-bounce propagation path:* For  $s = s'$ , the messages  $\gamma_{ss}^{(j)}(\mathbf{x}_n)$  propagate from the single-bounce PR related factor node  $q_S(\mathbf{x}_n, \underline{\mathbf{y}}_{s,n}^{(j)}, \underline{\boldsymbol{\beta}}_{ss,n}^{(j)}, \underline{\mathbf{a}}_{ss,n}^{(j)}; \mathbf{z}_n^{(j)})$  to the agent variable node  $\mathbf{x}_n$  are obtained as

$$\begin{aligned} \gamma_{ss}^{(j)}(\mathbf{x}_n) &= \sum_{\substack{\underline{r}_{ss,n}^{(j)} \in \{0,1\} \\ \underline{r}_{s,n}^{(j)} \in \{0,1\} \\ \underline{a}_{ss,n}^{(j)} \in \mathcal{M}_{0,n}^{(j)}}} \sum \eta(\underline{a}_{ss,n}^{(j)}) \iint \alpha(\underline{\mathbf{p}}_{s,\text{sfv}}^{(j)}, \underline{r}_{s,n}^{(j)}) \alpha(\underline{\mathbf{u}}_{ss,n}^{(j)}, \underline{r}_{ss,n}^{(j)}) \\ &\quad \times q_S(\mathbf{x}_n, \underline{\mathbf{p}}_{s,\text{sfv}}^{(j)}, \underline{r}_{s,n}^{(j)}, \underline{\mathbf{u}}_{ss,n}^{(j)}, \underline{r}_{ss,n}^{(j)}, \underline{\mathbf{a}}_{ss,n}^{(j)}; \mathbf{z}_n^{(j)}) d\underline{\mathbf{p}}_{s,\text{sfv}}^{(j)} d\underline{\mathbf{u}}_{ss,n}^{(j)} \\ &\quad + \eta(\underline{a}_{ss,n}^{(j)} = 0) \alpha_{ss,n}^{(j)} \underbrace{\left( \alpha_{s,n}^{(j)} + \int \alpha(\underline{\mathbf{p}}_{s,\text{sfv}}^{(j)}, 1) d\underline{\mathbf{p}}_{s,\text{sfv}}^{(j)} \right)}_{=1}. \end{aligned} \quad (33)$$

Finally, we obtain

$$\begin{aligned} \gamma_{ss}^{(j)}(\mathbf{x}_n) &= \sum_{\substack{\underline{a}_{ss,n}^{(j)} \in \mathcal{M}_{0,n}^{(j)}}} \eta(\underline{a}_{ss,n}^{(j)}) \iint \alpha(\underline{\mathbf{p}}_{s,\text{sfv}}^{(j)}, 1) \alpha(\underline{\mathbf{u}}_{ss,n}^{(j)}, 1) q_S(\mathbf{x}_n, \underline{\mathbf{p}}_{s,\text{sfv}}^{(j)}, 1, \underline{\mathbf{u}}_{ss,n}^{(j)}, 1, \underline{\mathbf{a}}_{ss,n}^{(j)}; \mathbf{z}_n^{(j)}) d\underline{\mathbf{p}}_{s,\text{sfv}}^{(j)} d\underline{\mathbf{u}}_{ss,n}^{(j)} \\ &\quad + \eta(\underline{a}_{ss,n}^{(j)} = 0) \alpha_{ss,n}^{(j)}. \end{aligned} \quad (34)$$

c) *Double-bounce propagation path:* For  $s \neq s'$ , the messages  $\gamma_{ss'}^{(j)}(\mathbf{x}_n)$  propagate from double-bounce PR related factor node  $q_D(\mathbf{x}_n, \underline{\mathbf{y}}_{s,n}^{(j)}, \underline{\mathbf{y}}_{s',n}^{(j)}, \underline{\mathbf{u}}_{ss',n}^{(j)}, \underline{\mathbf{a}}_{ss',n}^{(j)}; \mathbf{z}_n^{(j)})$  to the agent variable node  $\mathbf{x}_n$  are obtained as

$$\begin{aligned} \gamma_{ss'}^{(j)}(\mathbf{x}_n) &= \sum_{\substack{\underline{r}_{ss',n}^{(j)} \in \{0,1\} \\ \underline{r}_{s,n}^{(j)} \in \{0,1\} \\ \underline{r}_{s',n}^{(j)} \in \{0,1\} \\ \underline{a}_{ss',n}^{(j)} \in \mathcal{M}_{0,n}^{(j)}}} \sum \eta(\underline{a}_{ss',n}^{(j)}) \iiint \alpha(\underline{\mathbf{p}}_{s,\text{sfv}}^{(j)}, \underline{r}_{s,n}^{(j)}) \alpha(\underline{\mathbf{p}}_{s',\text{sfv}}^{(j)}, \underline{r}_{s',n}^{(j)}) \\ &\quad \times \alpha(\underline{\mathbf{u}}_{ss',n}^{(j)}, \underline{r}_{ss',n}^{(j)}) q_D(\mathbf{x}_n, \underline{\mathbf{p}}_{s,\text{sfv}}^{(j)}, 1, \underline{\mathbf{p}}_{s',\text{sfv}}^{(j)}, 1, \underline{\mathbf{u}}_{ss',n}^{(j)}, \underline{r}_{ss',n}^{(j)}, \underline{\mathbf{a}}_{ss',n}^{(j)}; \mathbf{z}_n^{(j)}) d\underline{\mathbf{p}}_{s,\text{sfv}}^{(j)} d\underline{\mathbf{p}}_{s',\text{sfv}}^{(j)} d\underline{\mathbf{u}}_{ss',n}^{(j)} \\ &= \sum_{\substack{\underline{a}_{ss',n}^{(j)} \in \mathcal{M}_{0,n}^{(j)}}} \eta(\underline{a}_{ss',n}^{(j)}) \iiint \alpha(\underline{\mathbf{p}}_{s,\text{sfv}}^{(j)}, 1) \alpha(\underline{\mathbf{p}}_{s',\text{sfv}}^{(j)}, 1) \alpha(\underline{\mathbf{u}}_{ss',n}^{(j)}, 1) \\ &\quad \times q_D(\mathbf{x}_n, \underline{\mathbf{p}}_{s,\text{sfv}}^{(j)}, 1, \underline{\mathbf{p}}_{s',\text{sfv}}^{(j)}, 1, \underline{\mathbf{u}}_{ss',n}^{(j)}, 1, \underline{\mathbf{a}}_{ss',n}^{(j)}; \mathbf{z}_n^{(j)}) d\underline{\mathbf{p}}_{s,\text{sfv}}^{(j)} d\underline{\mathbf{p}}_{s',\text{sfv}}^{(j)} d\underline{\mathbf{u}}_{ss',n}^{(j)} \\ &\quad + \eta(\underline{a}_{ss',n}^{(j)} = 0) \left( \alpha_{ss',n}^{(j)} \alpha_{s',n}^{(j)} \underbrace{\left( \alpha_{s,n}^{(j)} + \int \alpha(\underline{\mathbf{p}}_{s,\text{sfv}}^{(j)}, 1) d\underline{\mathbf{p}}_{s,\text{sfv}}^{(j)} \right)}_{=1} \right. \\ &\quad \left. + \alpha_{ss',n}^{(j)} \underbrace{\left( \alpha_{s,n}^{(j)} + \int \alpha(\underline{\mathbf{p}}_{s,\text{sfv}}^{(j)}, 1) d\underline{\mathbf{p}}_{s,\text{sfv}}^{(j)} \right)}_{=1} \int \alpha(\underline{\mathbf{p}}_{s',\text{sfv}}^{(j)}, 1) d\underline{\mathbf{p}}_{s',\text{sfv}}^{(j)} \right). \end{aligned} \quad (35)$$

Finally, we obtain

$$\begin{aligned} \gamma_{ss'}^{(j)}(\mathbf{x}_n) &= \eta(\underline{a}_{ss',n}^{(j)} = 0) \alpha_{ss',n}^{(j)} + \sum_{\substack{\underline{a}_{ss',n}^{(j)} \in \mathcal{M}_{0,n}^{(j)}}} \eta(\underline{a}_{ss',n}^{(j)}) \iiint \alpha(\underline{\mathbf{p}}_{s,\text{sfv}}^{(j)}, 1) \alpha(\underline{\mathbf{p}}_{s',\text{sfv}}^{(j)}, 1) \alpha(\underline{\mathbf{u}}_{ss',n}^{(j)}, 1) \\ &\quad \times q_D(\mathbf{x}_n, \underline{\mathbf{p}}_{s,\text{sfv}}^{(j)}, 1, \underline{\mathbf{p}}_{s',\text{sfv}}^{(j)}, 1, \underline{\mathbf{u}}_{ss',n}^{(j)}, 1, \underline{\mathbf{a}}_{ss',n}^{(j)}; \mathbf{z}_n^{(j)}) d\underline{\mathbf{p}}_{s,\text{sfv}}^{(j)} d\underline{\mathbf{p}}_{s',\text{sfv}}^{(j)} d\underline{\mathbf{u}}_{ss',n}^{(j)}. \end{aligned} \quad (36)$$

#### 6) Measurement Update for Legacy PSFVs:

a) *Single-bounce propagation path:* For  $s = s'$ , the messages  $\rho_{ss}(\mathbf{y}_{s,n}^{(j)})$  propagate from the factor node  $q_S(\mathbf{x}_n, \underline{\mathbf{y}}_{s,n}^{(j)}, \underline{\boldsymbol{\beta}}_{ss,n}^{(j)}, \underline{\mathbf{a}}_{ss,n}^{(j)}; \mathbf{z}_n^{(j)})$  to the PSFV variable node  $\mathbf{y}_{s,n}^{(j)}$  are obtained as

$$\begin{aligned} \rho_{ss}(\underline{\mathbf{p}}_{s,\text{sfv}}^{(j)}, \underline{r}_{s,n}^{(j)}) &= \sum_{\substack{\underline{r}_{ss,n}^{(j)} \in \{0,1\} \\ \underline{a}_{ss,n}^{(j)} \in \mathcal{M}_{0,n}^{(j)}}} \sum \eta(\underline{a}_{ss,n}^{(j)}) \iint \alpha(\mathbf{x}_n) \alpha(\underline{\mathbf{u}}_{ss,n}^{(j)}, \underline{r}_{ss,n}^{(j)}) q_S(\mathbf{x}_n, \underline{\mathbf{p}}_{s,\text{sfv}}^{(j)}, \underline{r}_{s,n}^{(j)}, \underline{\mathbf{u}}_{ss,n}^{(j)}, \underline{r}_{ss,n}^{(j)}, \underline{\mathbf{a}}_{ss,n}^{(j)}; \mathbf{z}_n^{(j)}) d\mathbf{x}_n d\underline{\mathbf{u}}_{ss,n}^{(j)}. \end{aligned} \quad (37)$$

We further obtain the messages for existing legacy PSFVs as

$$\begin{aligned}
\rho_{ss}(\underline{\mathbf{p}}_{s,\text{sfv}}^{(j)}, 1) &= \sum_{\underline{a}_{ss,n}^{(j)} \in \mathcal{M}_{0,n}^{(j)}} \eta(\underline{a}_{ss,n}^{(j)}) \iint \alpha(\mathbf{x}_n) \alpha(\underline{u}_{ss,n}^{(j)}, 1) q_{\text{S}}(\mathbf{x}_n, \underline{\mathbf{p}}_{s,\text{sfv}}^{(j)}, 1, \underline{u}_{ss,n}^{(j)}, 1, \underline{a}_{ss,n}^{(j)}; \mathbf{z}_n^{(j)}) d\mathbf{x}_n d\underline{u}_{ss,n}^{(j)} \\
&\quad + \eta(\underline{a}_{ss,n}^{(j)} = 0) \iint \alpha(\mathbf{x}_n) \alpha(\underline{u}_{ss,n}^{(j)}, 0) d\mathbf{x}_n d\underline{u}_{ss,n}^{(j)} \\
&= \sum_{\underline{a}_{ss,n}^{(j)} \in \mathcal{M}_{0,n}^{(j)}} \eta(\underline{a}_{ss,n}^{(j)}) \iint \alpha(\mathbf{x}_n) \alpha(\underline{u}_{ss,n}^{(j)}, 1) q_{\text{S}}(\mathbf{x}_n, \underline{\mathbf{p}}_{s,\text{sfv}}^{(j)}, 1, \underline{u}_{ss,n}^{(j)}, 1, \underline{a}_{ss,n}^{(j)}; \mathbf{z}_n^{(j)}) d\mathbf{x}_n d\underline{u}_{ss,n}^{(j)} \\
&\quad + \eta(\underline{a}_{ss,n}^{(j)} = 0) \alpha_{ss,n}^{(j)},
\end{aligned} \tag{38}$$

and the messages  $\rho_{ss}(\underline{\mathbf{p}}_{s,\text{sfv}}^{(j)}, 0) \triangleq \rho_{ss}^{(j)}$  for nonexistent legacy PSFVs as

$$\begin{aligned}
\rho_{ss}(\underline{\mathbf{p}}_{s,\text{sfv}}^{(j)}, 0) &= \eta(\underline{a}_{ss,n}^{(j)} = 0) \iint \alpha(\mathbf{x}_n) \alpha(\underline{u}_{ss,n}^{(j)}, 0) d\mathbf{x}_n d\underline{u}_{ss,n}^{(j)} \\
&= \eta(\underline{a}_{ss,n}^{(j)} = 0) \alpha_{ss,n}^{(j)}.
\end{aligned} \tag{39}$$

*b) Double-bounce propagation path:* For  $s \neq s'$ , the messages  $\rho_{ss'}(\mathbf{y}_{s,n}^{(j)})$  from the factor node  $q_{\text{D}}(\mathbf{x}_n, \mathbf{y}_{s,n}^{(j)}, \mathbf{y}_{s',n}^{(j)}, \underline{\beta}_{ss',n}^{(j)}, \underline{a}_{ss',n}^{(j)}; \mathbf{z}_n^{(j)})$  to the PSFV variable node  $\mathbf{y}_{s,n}^{(j)}$  are obtained as

$$\begin{aligned}
\rho_{ss'}(\underline{\mathbf{p}}_{s,\text{sfv}}^{(j)}, \underline{r}_{s,n}^{(j)}) &= \sum_{\underline{r}_{ss',n}^{(j)} \in \{0,1\}} \sum_{\underline{r}_{s',n}^{(j)} \in \{0,1\}} \sum_{\underline{a}_{ss',n}^{(j)} \in \mathcal{M}_{0,n}^{(j)}} \eta(\underline{a}_{ss',n}^{(j)}) \iiint \alpha(\mathbf{x}_n) \alpha(\underline{\mathbf{p}}_{s',\text{sfv}}^{(j)}, \underline{r}_{s',n}^{(j)}) \alpha(\underline{u}_{ss',n}^{(j)}, \underline{r}_{s',n}^{(j)}) \\
&\quad \times q_{\text{D}}(\mathbf{x}_n, \underline{\mathbf{p}}_{s,\text{sfv}}^{(j)}, \underline{r}_{s,n}^{(j)}, \underline{\mathbf{p}}_{s',\text{sfv}}^{(j)}, \underline{r}_{s',n}^{(j)}, \underline{u}_{ss',n}^{(j)}, \underline{r}_{s',n}^{(j)}, \underline{a}_{ss',n}^{(j)}; \mathbf{z}_n^{(j)}) d\mathbf{x}_n d\underline{\mathbf{p}}_{s',\text{sfv}}^{(j)} d\underline{u}_{ss',n}^{(j)}.
\end{aligned} \tag{40}$$

We further obtain the messages for existing legacy PSFVs as

$$\begin{aligned}
\rho_{ss'}(\underline{\mathbf{p}}_{s,\text{sfv}}^{(j)}, 1) &= \sum_{\underline{a}_{ss',n}^{(j)} \in \mathcal{M}_{0,n}^{(j)}} \eta(\underline{a}_{ss',n}^{(j)}) \iiint \alpha(\mathbf{x}_n) \alpha(\underline{\mathbf{p}}_{s',\text{sfv}}^{(j)}, 1) \alpha(\underline{u}_{ss',n}^{(j)}, 1) \\
&\quad \times q_{\text{D}}(\mathbf{x}_n, \underline{\mathbf{p}}_{s,\text{sfv}}^{(j)}, 1, \underline{\mathbf{p}}_{s',\text{sfv}}^{(j)}, 1, \underline{u}_{ss',n}^{(j)}, 1, \underline{a}_{ss',n}^{(j)}; \mathbf{z}_n^{(j)}) d\mathbf{x}_n d\underline{\mathbf{p}}_{s',\text{sfv}}^{(j)} d\underline{u}_{ss',n}^{(j)} \\
&\quad + \eta(\underline{a}_{ss',n}^{(j)} = 0) \alpha_{ss',n}^{(j)} \underbrace{\left( \alpha_{s',n}^{(j)} + \int \alpha(\underline{\mathbf{p}}_{s',\text{sfv}}^{(j)}, 1) d\underline{\mathbf{p}}_{s',\text{sfv}}^{(j)} \right)}_{=1} \\
&= \sum_{\underline{a}_{ss',n}^{(j)} \in \mathcal{M}_{0,n}^{(j)}} \eta(\underline{a}_{ss',n}^{(j)}) \iiint \alpha(\mathbf{x}_n) \alpha(\underline{\mathbf{p}}_{s',\text{sfv}}^{(j)}, 1) \alpha(\underline{u}_{ss',n}^{(j)}, 1) \\
&\quad \times q_{\text{D}}(\mathbf{x}_n, \underline{\mathbf{p}}_{s,\text{sfv}}^{(j)}, 1, \underline{\mathbf{p}}_{s',\text{sfv}}^{(j)}, 1, \underline{u}_{ss',n}^{(j)}, 1, \underline{a}_{ss',n}^{(j)}; \mathbf{z}_n^{(j)}) d\mathbf{x}_n d\underline{\mathbf{p}}_{s',\text{sfv}}^{(j)} d\underline{u}_{ss',n}^{(j)} \\
&\quad + \eta(\underline{a}_{ss',n}^{(j)} = 0) \alpha_{ss',n}^{(j)},
\end{aligned} \tag{41}$$

and the messages  $\rho_{ss'}(\underline{\mathbf{p}}_{s,\text{sfv}}^{(j)}, 0) \triangleq \rho_{ss'}^{(j)}$  for nonexistent legacy PSFVs as

$$\begin{aligned}
\rho_{ss'}(\underline{\mathbf{p}}_{s,\text{sfv}}^{(j)}, 0) &= \eta(\underline{a}_{ss',n}^{(j)} = 0) \alpha_{ss',n}^{(j)} \underbrace{\left( \alpha_{s',n}^{(j)} + \int \alpha(\underline{\mathbf{p}}_{s',\text{sfv}}^{(j)}, 1) d\underline{\mathbf{p}}_{s',\text{sfv}}^{(j)} \right)}_{=1} \\
&= \eta(\underline{a}_{ss',n}^{(j)} = 0) \alpha_{ss',n}^{(j)}.
\end{aligned} \tag{42}$$

The messages sent to the next PA  $\gamma(\underline{y}_{s,n}^{(j)}) \triangleq \gamma(\underline{p}_{s,\text{sfv}}^{(j)}, \underline{r}_{s,n}^{(j)})$  are given as

$$\gamma(\underline{p}_{s,\text{sfv}}^{(j)}, 1) = \alpha(\underline{p}_{s,\text{sfv}}^{(j)}, 1) \rho_{ss}(\underline{p}_{s,\text{sfv}}^{(j)}, 1) \prod_{s'=1, s' \neq s}^{S_n^{(j)}} \rho_{ss'}(\underline{p}_{s,\text{sfv}}^{(j)}, 1), \quad (43)$$

$$\gamma(\underline{p}_{s,\text{sfv}}^{(j)}, 0) \triangleq \gamma_{s,n}^{(j)} = \alpha(\underline{p}_{s,\text{sfv}}^{(j)}, 0) \rho_{ss}(\underline{p}_{s,\text{sfv}}^{(j)}, 0) \prod_{s'=1, s' \neq s}^{S_n^{(j)}} \rho_{ss'}. \quad (44)$$

7) *Measurement Update for New PSFVs*: The messages  $\phi(\underline{y}_{m,n}^{(j)}) \triangleq \phi(\underline{p}_{m,\text{sfv}}^{(j)}, \bar{r}_{m,n}^{(j)})$  sent from  $\bar{q}_N(\mathbf{x}_n, \underline{y}_{m,n}^{(j)}, \bar{\beta}_{m,n}^{(j)}, \bar{a}_{m,n}^{(j)}; \mathbf{z}_n^{(j)})$  to the new PR variable node  $\underline{y}_{m,n}^{(j)}$  are given as follows with  $\tilde{\mathcal{D}}_{0,n}^{(j)} \triangleq \{0, \tilde{\mathcal{D}}_n^{(j)}\}$ ,

$$\begin{aligned} & \phi(\underline{p}_{m,\text{sfv}}^{(j)}, \bar{r}_{m,n}^{(j)}) \\ &= \sum_{\bar{r}_{mm,n}^{(j)} \in \{0,1\}} \sum_{\bar{a}_{m,n}^{(j)} \in \tilde{\mathcal{D}}_{0,n}^{(j)}} \varsigma(\bar{a}_{m,n}^{(j)}) \iint \alpha(\mathbf{x}_n) \bar{q}_N(\mathbf{x}_n, \underline{p}_{m,\text{sfv}}^{(j)}, \bar{r}_{m,n}^{(j)}, \bar{u}_{mm,n}^{(j)}, \bar{r}_{mm,n}^{(j)}, \bar{a}_{m,n}^{(j)}; \mathbf{z}_n^{(j)}) d\mathbf{x}_n d\bar{u}_{mm,n}^{(j)}. \end{aligned} \quad (45)$$

We further obtain the messages  $\phi(\underline{p}_{m,\text{sfv}}^{(j)}, 1)$  for existing new PSFVs as

$$\phi(\underline{p}_{m,\text{sfv}}^{(j)}, 1) = \varsigma(\bar{a}_{m,n}^{(j)} = 0) \iint \alpha(\mathbf{x}_n) \bar{q}_N(\mathbf{x}_n, \underline{p}_{m,\text{sfv}}^{(j)}, 1, \bar{u}_{mm,n}^{(j)}, 1, 0; \mathbf{z}_n^{(j)}) d\mathbf{x}_n d\bar{u}_{mm,n}^{(j)}, \quad (46)$$

and the messages  $\phi(\underline{p}_{m,\text{sfv}}^{(j)}, 0) \triangleq \phi_{m,n}^{(j)}$  for nonexistent new PSFVs as

$$\begin{aligned} \phi(\underline{p}_{m,\text{sfv}}^{(j)}, 0) &= \sum_{\bar{a}_{m,n}^{(j)} \in \tilde{\mathcal{D}}_{0,n}^{(j)}} \varsigma(\bar{a}_{m,n}^{(j)}) \underbrace{\left( \iint \alpha(\mathbf{x}_n) f_D(\underline{p}_{m,\text{sfv}}^{(j)}) f_D(\bar{u}_{mm,n}^{(j)}) d\mathbf{x}_n d\bar{u}_{mm,n}^{(j)} \right)}_{=1} \\ &= \sum_{\bar{a}_{m,n}^{(j)} \in \tilde{\mathcal{D}}_{0,n}^{(j)}} \varsigma(\bar{a}_{m,n}^{(j)}). \end{aligned} \quad (47)$$

8) *Measurement Update for Legacy PRs*:

a) *LoS propagation path*: The messages  $\kappa(\underline{\beta}_{00,n}^{(j)}) \triangleq \kappa(\underline{u}_{00,n}^{(j)}, \underline{r}_{00,n}^{(j)})$  sent from the LoS PR related factor node  $\underline{q}_P(\mathbf{x}_n, \underline{\beta}_{00,n}^{(j)}, \underline{a}_{00,n}^{(j)}; \mathbf{z}_n^{(j)})$  to the LoS PR state variable node  $\underline{\beta}_{00,n}^{(j)}$  are obtained as

$$\kappa(\underline{u}_{00,n}^{(j)}, 1) = \sum_{\underline{a}_{00,n}^{(j)} \in \mathcal{M}_{0,n}^{(j)}} \eta(\underline{a}_{00,n}^{(j)}) \int \alpha(\mathbf{x}_n) \underline{q}_P(\mathbf{x}_n, \underline{u}_{00,n}^{(j)}, 1, \underline{a}_{00,n}^{(j)}; \mathbf{z}_n^{(j)}) d\mathbf{x}_n, \quad (48)$$

$$\kappa(\underline{u}_{00,n}^{(j)}, 0) \triangleq \kappa_{00,n}^{(j)} = \eta(\underline{a}_{00,n}^{(j)} = 0) \int \alpha(\mathbf{x}_n) \delta(\underline{a}_{00,n}^{(j)} = 0) d\mathbf{x}_n = \eta(\underline{a}_{00,n}^{(j)} = 0). \quad (49)$$

b) *Single-bounce propagation path*: For  $s = s'$ , the messages  $\kappa(\underline{\beta}_{ss,n}^{(j)}) \triangleq \kappa(\underline{u}_{ss,n}^{(j)}, \underline{r}_{ss,n}^{(j)})$  sent from the single-bounce PR related factor node  $\underline{q}_S(\mathbf{x}_n, \underline{y}_{s,n}^{(j)}, \underline{\beta}_{ss,n}^{(j)}, \underline{a}_{ss,n}^{(j)}; \mathbf{z}_n^{(j)})$  to the single-bounce PR state variable node  $\underline{\beta}_{ss,n}^{(j)}$  are obtained as

$$\begin{aligned} \kappa(\underline{u}_{ss,n}^{(j)}, 1) &= \sum_{\underline{r}_{s,n}^{(j)} \in \{0,1\}} \sum_{\underline{a}_{ss,n}^{(j)} \in \mathcal{M}_{0,n}^{(j)}} \eta(\underline{a}_{ss,n}^{(j)}) \iint \alpha(\mathbf{x}_n) \alpha(\underline{p}_{s,\text{sfv}}^{(j)}, \underline{r}_{s,n}^{(j)}) \\ &\quad \times \underline{q}_S(\mathbf{x}_n, \underline{p}_{s,\text{sfv}}^{(j)}, \underline{r}_{s,n}^{(j)}, \underline{u}_{ss,n}^{(j)}, \underline{r}_{ss,n}^{(j)}, \underline{a}_{ss,n}^{(j)}; \mathbf{z}_n^{(j)}) d\mathbf{x}_n d\underline{p}_{s,\text{sfv}}^{(j)}. \end{aligned} \quad (50)$$

We further obtain the messages for existing legacy PRs as

$$\kappa(\underline{u}_{ss,n}^{(j)}, 1) = \sum_{\underline{a}_{ss,n}^{(j)} \in \mathcal{M}_{0,n}^{(j)}} \eta(\underline{a}_{ss,n}^{(j)}) \iint \alpha(\mathbf{x}_n) \alpha_s(\underline{p}_{s,\text{sfv}}^{(j)}, 1) \underline{q}_S(\mathbf{x}_n, \underline{p}_{s,\text{sfv}}^{(j)}, 1, \underline{u}_{ss,n}^{(j)}, 1, \underline{a}_{ss,n}^{(j)}; \mathbf{z}_n^{(j)}) d\mathbf{x}_n d\underline{p}_{s,\text{sfv}}^{(j)}, \quad (51)$$

and the messages  $\kappa(\underline{u}_{ss,n}^{(j)}, 0) \triangleq \kappa_{ss,n}^{(j)}$  for nonexistent legacy PRs as

$$\kappa(\underline{u}_{ss,n}^{(j)}, 0) = \eta(\underline{a}_{ss,n}^{(j)} = 0) \underbrace{\left( \alpha_{s,n}^{(j)} + \int \alpha(\underline{p}_{s,\text{sfv}}^{(j)}, 1) d\underline{p}_{s,\text{sfv}}^{(j)} \right)}_{=1} = \eta(\underline{a}_{ss,n}^{(j)} = 0). \quad (52)$$

c) *Double-bounce propagation path*: For  $s \neq s'$ , the messages  $\kappa(\underline{\beta}_{ss',n}^{(j)}) \triangleq \kappa(\underline{u}_{ss',n}^{(j)}, \underline{r}_{ss',n}^{(j)})$  sent from the double-bounce PR related factor node  $\underline{q}_D(\underline{x}_n, \underline{y}_{s,n}^{(j)}, \underline{y}_{s',n}^{(j)}, \underline{\beta}_{ss',n}^{(j)}, \underline{a}_{ss',n}^{(j)}; \underline{z}_n^{(j)})$  to the legacy PR state variable node  $\underline{\beta}_{ss',n}^{(j)}$  are obtained as

$$\begin{aligned} \kappa(\underline{u}_{ss',n}^{(j)}, \underline{r}_{ss',n}^{(j)}) &= \sum_{\substack{\underline{r}_{s,n}^{(j)} \in \{0,1\} \\ \underline{r}_{s',n}^{(j)} \in \{0,1\}}} \sum_{\substack{\underline{a}_{ss',n}^{(j)} \in \mathcal{M}_{0,n}^{(j)}}} \eta(\underline{a}_{ss',n}^{(j)}) \iiint \alpha(\underline{x}_n) \alpha(\underline{p}_{s,\text{sfv}}^{(j)}, \underline{r}_{s,n}^{(j)}) \alpha(\underline{p}_{s',\text{sfv}}^{(j)}, \underline{r}_{s',n}^{(j)}) \\ &\times \underline{q}_D(\underline{x}_n, \underline{p}_{s,\text{sfv}}^{(j)}, \underline{r}_{s,n}^{(j)}, \underline{p}_{s',\text{sfv}}^{(j)}, \underline{r}_{s',n}^{(j)}, \underline{u}_{ss',n}^{(j)}, \underline{r}_{ss',n}^{(j)}, \underline{a}_{ss',n}^{(j)}; \underline{z}_n^{(j)}) d\underline{x}_n d\underline{p}_{s,\text{sfv}}^{(j)} d\underline{p}_{s',\text{sfv}}^{(j)}. \end{aligned} \quad (53)$$

We further obtain the messages  $\kappa(\underline{u}_{ss',n}^{(j)}, 1)$  for existing legacy PRs as

$$\begin{aligned} \kappa(\underline{u}_{ss',n}^{(j)}, 1) &= \sum_{\substack{\underline{a}_{ss',n}^{(j)} \in \mathcal{M}_{0,n}^{(j)}}} \eta(\underline{a}_{ss',n}^{(j)}) \iiint \alpha(\underline{x}_n) \alpha(\underline{p}_{s,\text{sfv}}^{(j)}, 1) \alpha(\underline{p}_{s',\text{sfv}}^{(j)}, 1) \\ &\times \underline{q}_D(\underline{x}_n, \underline{p}_{s,\text{sfv}}^{(j)}, 1, \underline{p}_{s',\text{sfv}}^{(j)}, 1, \underline{u}_{ss',n}^{(j)}, 1, \underline{a}_{ss',n}^{(j)}; \underline{z}_n^{(j)}) d\underline{x}_n d\underline{p}_{s,\text{sfv}}^{(j)} d\underline{p}_{s',\text{sfv}}^{(j)}, \end{aligned} \quad (54)$$

and the messages  $\kappa(\underline{u}_{ss',n}^{(j)}, 0) \triangleq \kappa_{ss',n}^{(j)}$  for nonexistent legacy PRs as

$$\begin{aligned} \kappa(\underline{u}_{ss',n}^{(j)}, 0) &= \eta(\underline{a}_{ss',n}^{(j)} = 0) \underbrace{\left( \int \alpha(\underline{p}_{s,\text{sfv}}^{(j)}, 1) d\underline{p}_{s,\text{sfv}}^{(j)} \int \alpha(\underline{p}_{s',\text{sfv}}^{(j)}, 1) d\underline{p}_{s',\text{sfv}}^{(j)} + \alpha_{s,n}^{(j)} \int \alpha(\underline{p}_{s',\text{sfv}}^{(j)}, 1) d\underline{p}_{s',\text{sfv}}^{(j)} \right.} \\ &\quad \left. + \alpha_{s',n}^{(j)} \int \alpha(\underline{p}_{s,\text{sfv}}^{(j)}, 1) d\underline{p}_{s,\text{sfv}}^{(j)} + \alpha_{s,n}^{(j)} \alpha_{s',n}^{(j)} \right)}_{=1} \\ &= \eta(\underline{a}_{ss',n}^{(j)} = 0). \end{aligned} \quad (55)$$

Based on the messages above, the messages  $\gamma(\underline{\beta}_{ss',n}^{(j)}) \triangleq \gamma(\underline{u}_{ss',n}^{(j)}, \underline{r}_{ss',n}^{(j)})$  sent to the next time step  $n+1$  are computed as

$$\gamma(\underline{u}_{ss',n}^{(j)}, 1) = \alpha(\underline{u}_{ss',n}^{(j)}, 1) \kappa(\underline{u}_{ss',n}^{(j)}, 1), \quad (56)$$

$$\gamma(\underline{u}_{ss',n}^{(j)}, 0) = \alpha(\underline{u}_{ss',n}^{(j)}, 0) \kappa(\underline{u}_{ss',n}^{(j)}, 0). \quad (57)$$

9) *Measurement Update for New PRs*: The messages  $\kappa(\underline{\beta}_{mm,n}^{(j)}) \triangleq \kappa(\underline{u}_{mm,n}^{(j)}, \underline{r}_{mm,n}^{(j)})$  sent from the factor node  $\bar{q}_N(\underline{x}_n, \bar{\underline{y}}_{m,n}^{(j)}, \bar{\underline{\beta}}_{m,n}^{(j)}, \bar{\underline{a}}_{m,n}^{(j)}; \underline{z}_n^{(j)})$  to the new PR variable node  $\bar{\underline{\beta}}_{mm,n}^{(j)}$  are given by

$$\begin{aligned} \kappa(\underline{u}_{mm,n}^{(j)}, 1) &= \sum_{\substack{\bar{\underline{r}}_{m,n}^{(j)} \in \{0,1\}}} \sum_{\substack{\bar{\underline{a}}_{m,n}^{(j)} \in \bar{\mathcal{D}}_{0,n}^{(j)}}} \varsigma(\bar{\underline{a}}_{m,n}^{(j)}) \iiint \alpha(\underline{x}_n) \\ &\times \bar{q}_N(\underline{x}_n, \bar{\underline{p}}_{m,\text{sfv}}^{(j)}, \bar{\underline{r}}_{m,n}^{(j)}, \bar{\underline{u}}_{mm,n}^{(j)}, \bar{\underline{r}}_{mm,n}^{(j)}, \bar{\underline{a}}_{m,n}^{(j)}; \underline{z}_n^{(j)}) d\underline{x}_n d\bar{\underline{p}}_{m,\text{sfv}}^{(j)}. \end{aligned} \quad (58)$$

We further obtain the messages  $\kappa(\underline{u}_{mm,n}^{(j)}, 1)$  for existing new PRs as

$$\kappa(\underline{u}_{mm,n}^{(j)}, 1) = \varsigma(\bar{\underline{a}}_{m,n}^{(j)} = 0) \iiint \alpha(\underline{x}_n) \bar{q}_N(\underline{x}_n, \bar{\underline{p}}_{m,\text{sfv}}^{(j)}, 1, \bar{\underline{u}}_{mm,n}^{(j)}, 1, 0; \underline{z}_n^{(j)}) d\underline{x}_n d\bar{\underline{p}}_{m,\text{sfv}}^{(j)}, \quad (59)$$

and the messages  $\kappa(\underline{u}_{mm,n}^{(j)}, 0) \triangleq \kappa_{mm,n}^{(j)}$  for nonexistent new PRs as

$$\begin{aligned}\kappa(\underline{u}_{mm,n}^{(j)}, 0) &= \sum_{\bar{a}_{m,n}^{(j)} \in \bar{\mathcal{D}}_{0,n}^{(j)}} \varsigma(\bar{a}_{m,n}^{(j)}) \underbrace{\left( \iint \alpha(\mathbf{x}_n) f_D(\bar{\mathbf{p}}_{m,\text{sfv}}^{(j)}) d\mathbf{x}_n d\bar{\mathbf{p}}_{m,\text{sfv}}^{(j)} \right)}_{=1} \\ &= \sum_{\bar{a}_{m,n}^{(j)} \in \bar{\mathcal{D}}_{0,n}^{(j)}} \varsigma(\bar{a}_{m,n}^{(j)}).\end{aligned}\quad (60)$$

### C. Belief Calculation

After calculating the messages for all PAs, the belief  $\tilde{f}(\mathbf{x}_n)$  of the agent state approximating  $f(\mathbf{x}_n | \mathbf{z}_{1:n})$  is given by

$$\tilde{f}(\mathbf{x}_n) = C_n \alpha(\mathbf{x}_n) \prod_{(s,s') \in \mathcal{D}_n^{(j)}} \gamma_{ss'}^{(j)}(\mathbf{x}_n) \prod_{j=1}^J \gamma_{00}^{(j)}(\mathbf{x}_n), \quad (61)$$

with the normalization constant

$$C_n = \left( \int \alpha(\mathbf{x}_n) \prod_{(s,s') \in \mathcal{D}_n^{(j)}} \gamma_{ss'}^{(j)}(\mathbf{x}_n) \prod_{j=1}^J \gamma_{00}^{(j)}(\mathbf{x}_n) d\mathbf{x}_n \right)^{-1}. \quad (62)$$

The beliefs of legacy PSFVs  $\tilde{f}(\underline{\mathbf{y}}_{s,n}^{(j)}) \triangleq \tilde{f}(\underline{\mathbf{p}}_{s,\text{sfv}}^{(j)}, \underline{\mathbf{r}}_{s,n}^{(j)})$  with  $s \in \mathcal{S}_n^{(j)}$  are given by

$$\tilde{f}(\underline{\mathbf{y}}_{s,n}^{(j)}) = \underline{C}_{s,n} \gamma(\underline{\mathbf{y}}_{s,n}^{(j)}) \quad (63)$$

with the normalization constant  $\underline{C}_{s,n} = \left( \int \underline{\mathbf{y}}_{s,n}^{(j)} d\underline{\mathbf{y}}_{s,n}^{(j)} \right)^{-1}$ . Similarly, the beliefs of new PSFVs  $\tilde{f}(\bar{\mathbf{y}}_{m,n}^{(j)}) \triangleq \tilde{f}(\bar{\mathbf{p}}_{m,\text{sfv}}^{(j)}, \bar{\mathbf{r}}_{m,n}^{(j)})$  with  $m \in \mathcal{M}_n^{(j)}$  are given by

$$\tilde{f}(\bar{\mathbf{y}}_{m,n}^{(j)}) = \bar{C}_{m,n} \phi(\bar{\mathbf{y}}_{m,n}^{(j)}), \quad (64)$$

with the normalization constant  $\bar{C}_{m,n} = \left( \int \phi(\bar{\mathbf{y}}_{m,n}^{(j)}) d\bar{\mathbf{y}}_{m,n}^{(j)} \right)^{-1}$ .

At each PA  $j$ , the beliefs  $\tilde{f}(\underline{\boldsymbol{\beta}}_{ss',n}^{(j)}) \triangleq \tilde{f}(\underline{\mathbf{u}}_{ss',n}^{(j)}, \underline{\mathbf{r}}_{ss',n}^{(j)})$  of legacy PRs  $(s,s')' \in \tilde{\mathcal{D}}_n^{(j)}$  are given by

$$\tilde{f}(\underline{\boldsymbol{\beta}}_{ss',n}^{(j)}) = \underline{C}_{ss',n}^{(j)} \gamma(\underline{\boldsymbol{\beta}}_{ss',n}^{(j)}), \quad (65)$$

with the normalization constant  $\underline{C}_{ss',n}^{(j)} = \left( \int \underline{\boldsymbol{\beta}}_{ss',n}^{(j)} d\underline{\boldsymbol{\beta}}_{ss',n}^{(j)} \right)^{-1}$ . Similarly, the beliefs  $\tilde{f}(\bar{\boldsymbol{\beta}}_{mm,n}^{(j)}) \triangleq \tilde{f}(\bar{\mathbf{u}}_{mm,n}^{(j)}, \bar{\mathbf{r}}_{mm,n}^{(j)})$  of new PRs are given by

$$\tilde{f}(\bar{\boldsymbol{\beta}}_{mm,n}^{(j)}) = \bar{C}_{mm,n}^{(j)} \kappa(\bar{\boldsymbol{\beta}}_{mm,n}^{(j)}), \quad (66)$$

with the normalization constant  $\bar{C}_{mm,n}^{(j)} = \left( \int \bar{\boldsymbol{\beta}}_{mm,n}^{(j)} d\bar{\boldsymbol{\beta}}_{mm,n}^{(j)} \right)^{-1}$ . The normalization constants  $C_n$ ,  $\underline{C}_{s,n}$ ,  $\bar{C}_{m,n}$ ,  $\underline{C}_{ss',n}^{(j)}$ ,  $\bar{C}_{mm,n}^{(j)}$  ensure that the beliefs are valid probability distributions.

As the integrations involved in the message and belief calculations cannot be obtained analytically, we employ a computationally efficient, sequential, particle-based, message-passing implementation, as outlined in [2], [4], [5]. Specifically, we adopt a “stacked state” approach comprising the agent state, the PSFV states, and the PR states, as detailed in [5], [6]. This approach leads to complexity that scales linearly with the number of particles. The supplementary material of [5] provides a comprehensive description of the weight calculations when using “stacked states”.

## REFERENCES

- [1] X. Li, B. Deutschmann, E. Leitingner, and F. Meyer, "Adaptive multipath-based SLAM for distributed MIMO systems," 2025, arXiv.
- [2] E. Leitingner, A. Venus, B. Teague, and F. Meyer, "Data fusion for multipath-based SLAM: Combining information from multiple propagation paths," *IEEE Trans. Signal Process.*, vol. 71, pp. 4011–4028, Sep. 2023.
- [3] F. Meyer, T. Kropfreiter, J. L. Williams, R. Lau, F. Hlawatsch, P. Braca, and M. Z. Win, "Message passing algorithms for scalable multitarget tracking," *Proc. IEEE*, vol. 106, no. 2, pp. 221–259, Feb. 2018.
- [4] F. Meyer, P. Braca, P. Willett, and F. Hlawatsch, "A scalable algorithm for tracking an unknown number of targets using multiple sensors," *IEEE Trans. Signal Process.*, vol. 65, no. 13, pp. 3478–3493, July 2017.
- [5] A. Venus, E. Leitingner, S. Tertinek, F. Meyer, and K. Witrisal, "Graph-based simultaneous localization and bias tracking," *IEEE Trans. Wirel. Commun.*, vol. 23, no. 10, pp. 13 141–13 158, May 2024.
- [6] F. Meyer, O. Hlinka, H. Wymeersch, E. Riegler, and F. Hlawatsch, "Distributed localization and tracking of mobile networks including noncooperative objects," *IEEE Trans. Signal Inf. Process. Net.*, vol. 2, no. 1, pp. 57–71, Mar. 2016.
